# Supplementary material for: Differentiable Parsing and Visual Grounding of Natural Language Instructions for Object Placement
Source: arXiv:2210.00215 source file (2023-03-13)
Supplement: Supplementary file 1 [file 6_appendix.tex]

\appendix
\begin{center}
    \textbf{\LARGE Errors and Updates}
\end{center}

We apologize that we made a mistake when recording the experimental results of CLIPort in Table 2 of the paper (shown in Figure \ref{fig:error}). The updated version of the experimental results is illustrated in Table \ref{table:res1_latest}. Specifically, the rows in red are the experimental results after update. 

\begin{figure}[h]
    \centering
    \includegraphics[width=\textwidth]{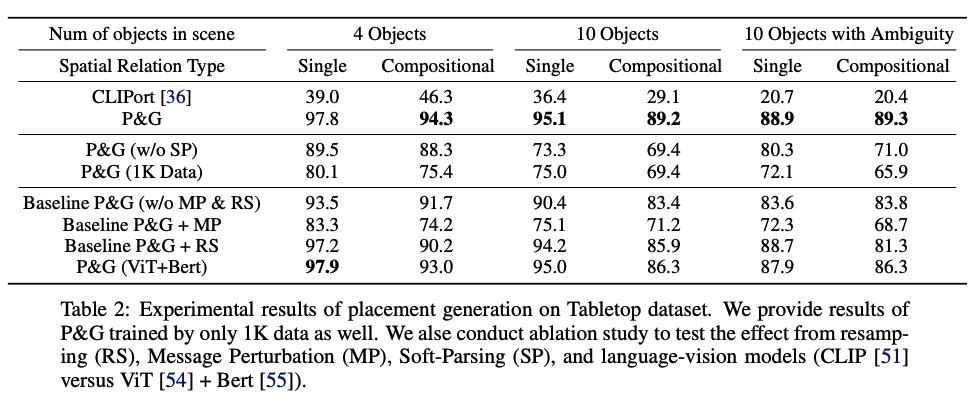}
    \caption{Original Results with Error.}
    \label{fig:error}
\end{figure}

\begin{table*}[h]
\footnotesize
\centering
\makebox[\textwidth][c]{
\begin{tabular}{P{40mm}P{11mm}P{18mm}P{11mm}P{18mm}P{11mm}P{18mm}}
    \toprule
    {\footnotesize Num of objects in scene} & 
    \multicolumn{2}{c}{\footnotesize 4 Objects} & 
    \multicolumn{2}{c}{\footnotesize 10 Objects} & 
    \multicolumn{2}{c}{\footnotesize 10 Objects with Ambiguity} \\ \cmidrule(lr){1-1}\cmidrule(lr){2-3}\cmidrule(lr){4-5}\cmidrule(lr){6-7}
    {Spatial Relation Type}&{\footnotesize Single} &{\footnotesize Compositional} &{\footnotesize Single} &{\footnotesize Compositional} &{\footnotesize Single} &{\footnotesize Compositional} \\ \cmidrule(lr){1-7} 
    %------
    \rowcolor{red!10}CLIPort~\cite{shridhar2021cliport} & 92.3  & 83.1  & 84.1  & 77.5  & 82.0  & 78.1   \\
    P\&G & 97.8  & \textbf{94.3}  & \textbf{95.1}  & \textbf{89.2}  & \textbf{88.9}  & \textbf{89.3}    \\
    \cmidrule(lr){1-7} 
    P\&G (w/o SP) & 89.5  & 88.3  & 73.3  & 69.4  & 80.3  & 71.0   \\
    P\&G (1K Data) & 80.1  & 75.4  & 75.0  & 69.4  & 72.1  & 65.9   \\
    \cmidrule(lr){1-7} 
    Baseline P\&G (w/o MP \& RS) & 93.5  & 91.7  & 90.4  & 83.4  & 83.6  & 83.8    \\
    Baseline P\&G + MP & 83.3  & 74.2  & 75.1  & 71.2  & 72.3  & 68.7    \\
    Baseline P\&G + RS & 97.2  & 90.2  & 94.2  & 85.9  & 88.7  & 81.3    \\
    P\&G (ViT+Bert) & \textbf{97.9}  & 93.0  & 95.0  & 86.3  & 87.9  & 86.3   \\
    \bottomrule
\end{tabular}}
\caption{The updated results.}
\label{table:res1_latest}
\end{table*}

% \textbf{\Large {\color{red} Apology}: we are sorry that the experimental results for CLIPort in the paper have some mistakes. The latest experimental results are attached in Appendix \ref{app:results}}

\clearpage
\newpage
