# Supplementary material for: Differentiable Parsing and Visual Grounding of Natural Language Instructions for Object Placement
Source: arXiv:2210.00215 source file (2023-03-13)
Supplement: Supplementary file 2 [file 6_appendix_.tex]

\appendices 

\section{Tabletop Dataset}
\label{app:dataset}

We extend the dataset from \href{https://bit.ly/TableSetData}{\bf\color{blue}{bit.ly/TableSetData}} with randomly sampled objects and generate placement from several sampled spatial relations. The dataset will be released in our website at \href{https://bit.ly/ParaGonProj}{\bf\color{blue} bit.ly/ParaGonProj}. 

\subsection{Objects}

We sample 50 dining objects with different classes, colors, and shapes, including forks, knives, spoons, plates, wine cups, water cups, and napkin cloths. The visualization of objects is in Fig. 5 (a).

\subsection{Language Expressions}

Our dataset draws samples from commonly used spatial relations with various language expressions. The spatial relations includes left, right, front, behind, on top of, and their compositions. We also have ternary spatial relation ``between''. The language expressions for each spatial relations are illustrated in Table \ref{app:tab_rel}.

\begin{table*}[]
\centering
\caption{Spatial relations and their language expressions in Tabletop Dataset.}
\begin{tabular}{@{}llll@{}}
\toprule
Spatial Relations &
  Language Expressions &
  Spatial Relations &
  Language Expressions \\ \midrule
Left &
  \begin{tabular}[c]{@{}l@{}}``to the left of''\\ ``to the left side of''\\ ``to the left hand side of''\end{tabular} &
  Front Right &
  \begin{tabular}[c]{@{}l@{}}``to the lower right of''\\ ``to the lower right side of''\\ ``to the lower right corner of''\\ ``to the front right of''\end{tabular} \\ \midrule
Right &
  \begin{tabular}[c]{@{}l@{}}``to the right of''\\ ``to the right side of''\\ ``to the right hand side of''\end{tabular} &
  Behind Left &
  \begin{tabular}[c]{@{}l@{}}``to the upper left of''\\ ``to the upper left side of''\\ ``to the upper left corner of''\end{tabular} \\ \midrule
Front &
  \begin{tabular}[c]{@{}l@{}}``in front of''\\ ``to the lower side of''\end{tabular} &
  Behind Right &
  \begin{tabular}[c]{@{}l@{}}``to the upper right of''\\ ``to the upper right side of''\\ ``to the upper right corner of''\end{tabular} \\ \midrule
Behind &
  \begin{tabular}[c]{@{}l@{}}``behind''\\ ``to the upper side of''\end{tabular} &
  on top of &
  \begin{tabular}[c]{@{}l@{}}``on''\\ ``above''\\ ``on top of''\\ ``on the center of''\end{tabular} \\ \midrule
Front Left &
  \begin{tabular}[c]{@{}l@{}}``to the lower left of''\\ ``to the lower left side of''\\ ``to the lower left corner of''\\ ``to the front left of''\end{tabular} &
   &
   \\ \bottomrule
\end{tabular}
\vspace{3mm}
\label{app:tab_rel}
\end{table*}

\subsection{Data Generation}

\subsubsection{Instruction Generation}

We generate the instructions according to language templates. The template for tasks with single spatial relation is illustrated below:
\begin{align}
    &\text{[verb phrase]} + \text{[subject phrase]} \\&+ \text{[spatial relation phrase]} + \text{[object phrase]}.
\end{align}
If the language instruction contains compositional spatial relations, the template is:
\begin{align}
    &\text{[verb phrase]} + \text{[subject phrase]} \\+& \text{[spatial relation phrase 1]} + \text{[object phrase 1]}\\+&\text{``and''}+ \text{[spatial relation prhase 2]} + \text{[object phrase 2]}.
\end{align}
The spatial relations are sampled from Table \ref{app:tab_rel}, and the subject phrases and object phrases are sampled according to the object class, object colors, and shapes, such as ``yellow square plate''. We sample the verb phrases uniformly as random from ``put'', ``place'', and ``move''.

\subsubsection{Image Generation}

\begin{itemize}
  \item \textbf{Camera Setup.} We use four cameras to capture the visual observation. Similar to the Raven simulator, there are three RGB-D cameras with resolutions of $640\times 480$ that are placed on the rectangular table's top, left, and right, pointing towards the center (see (b), (c), and (d) in Figure \ref{app:fig_camera}). We also have an RGB camera with a resolution of $640\times 640$ placed at the top of the table (see (a) in Figure \ref{app:fig_camera} for the example picture).
  \item \textbf{Rendering.} We use NVISII as the rendering interface to get the photorealistic pictures of the visual scene. We randomly sample the position of the lights and their colors to add difficulties. In addition, due to the random lighting conditions, the visual scenes contain various light reflections, hampering the visual grounding of natural language. 
\end{itemize}

\begin{figure}
  \centering
  \includegraphics[width=\columnwidth]{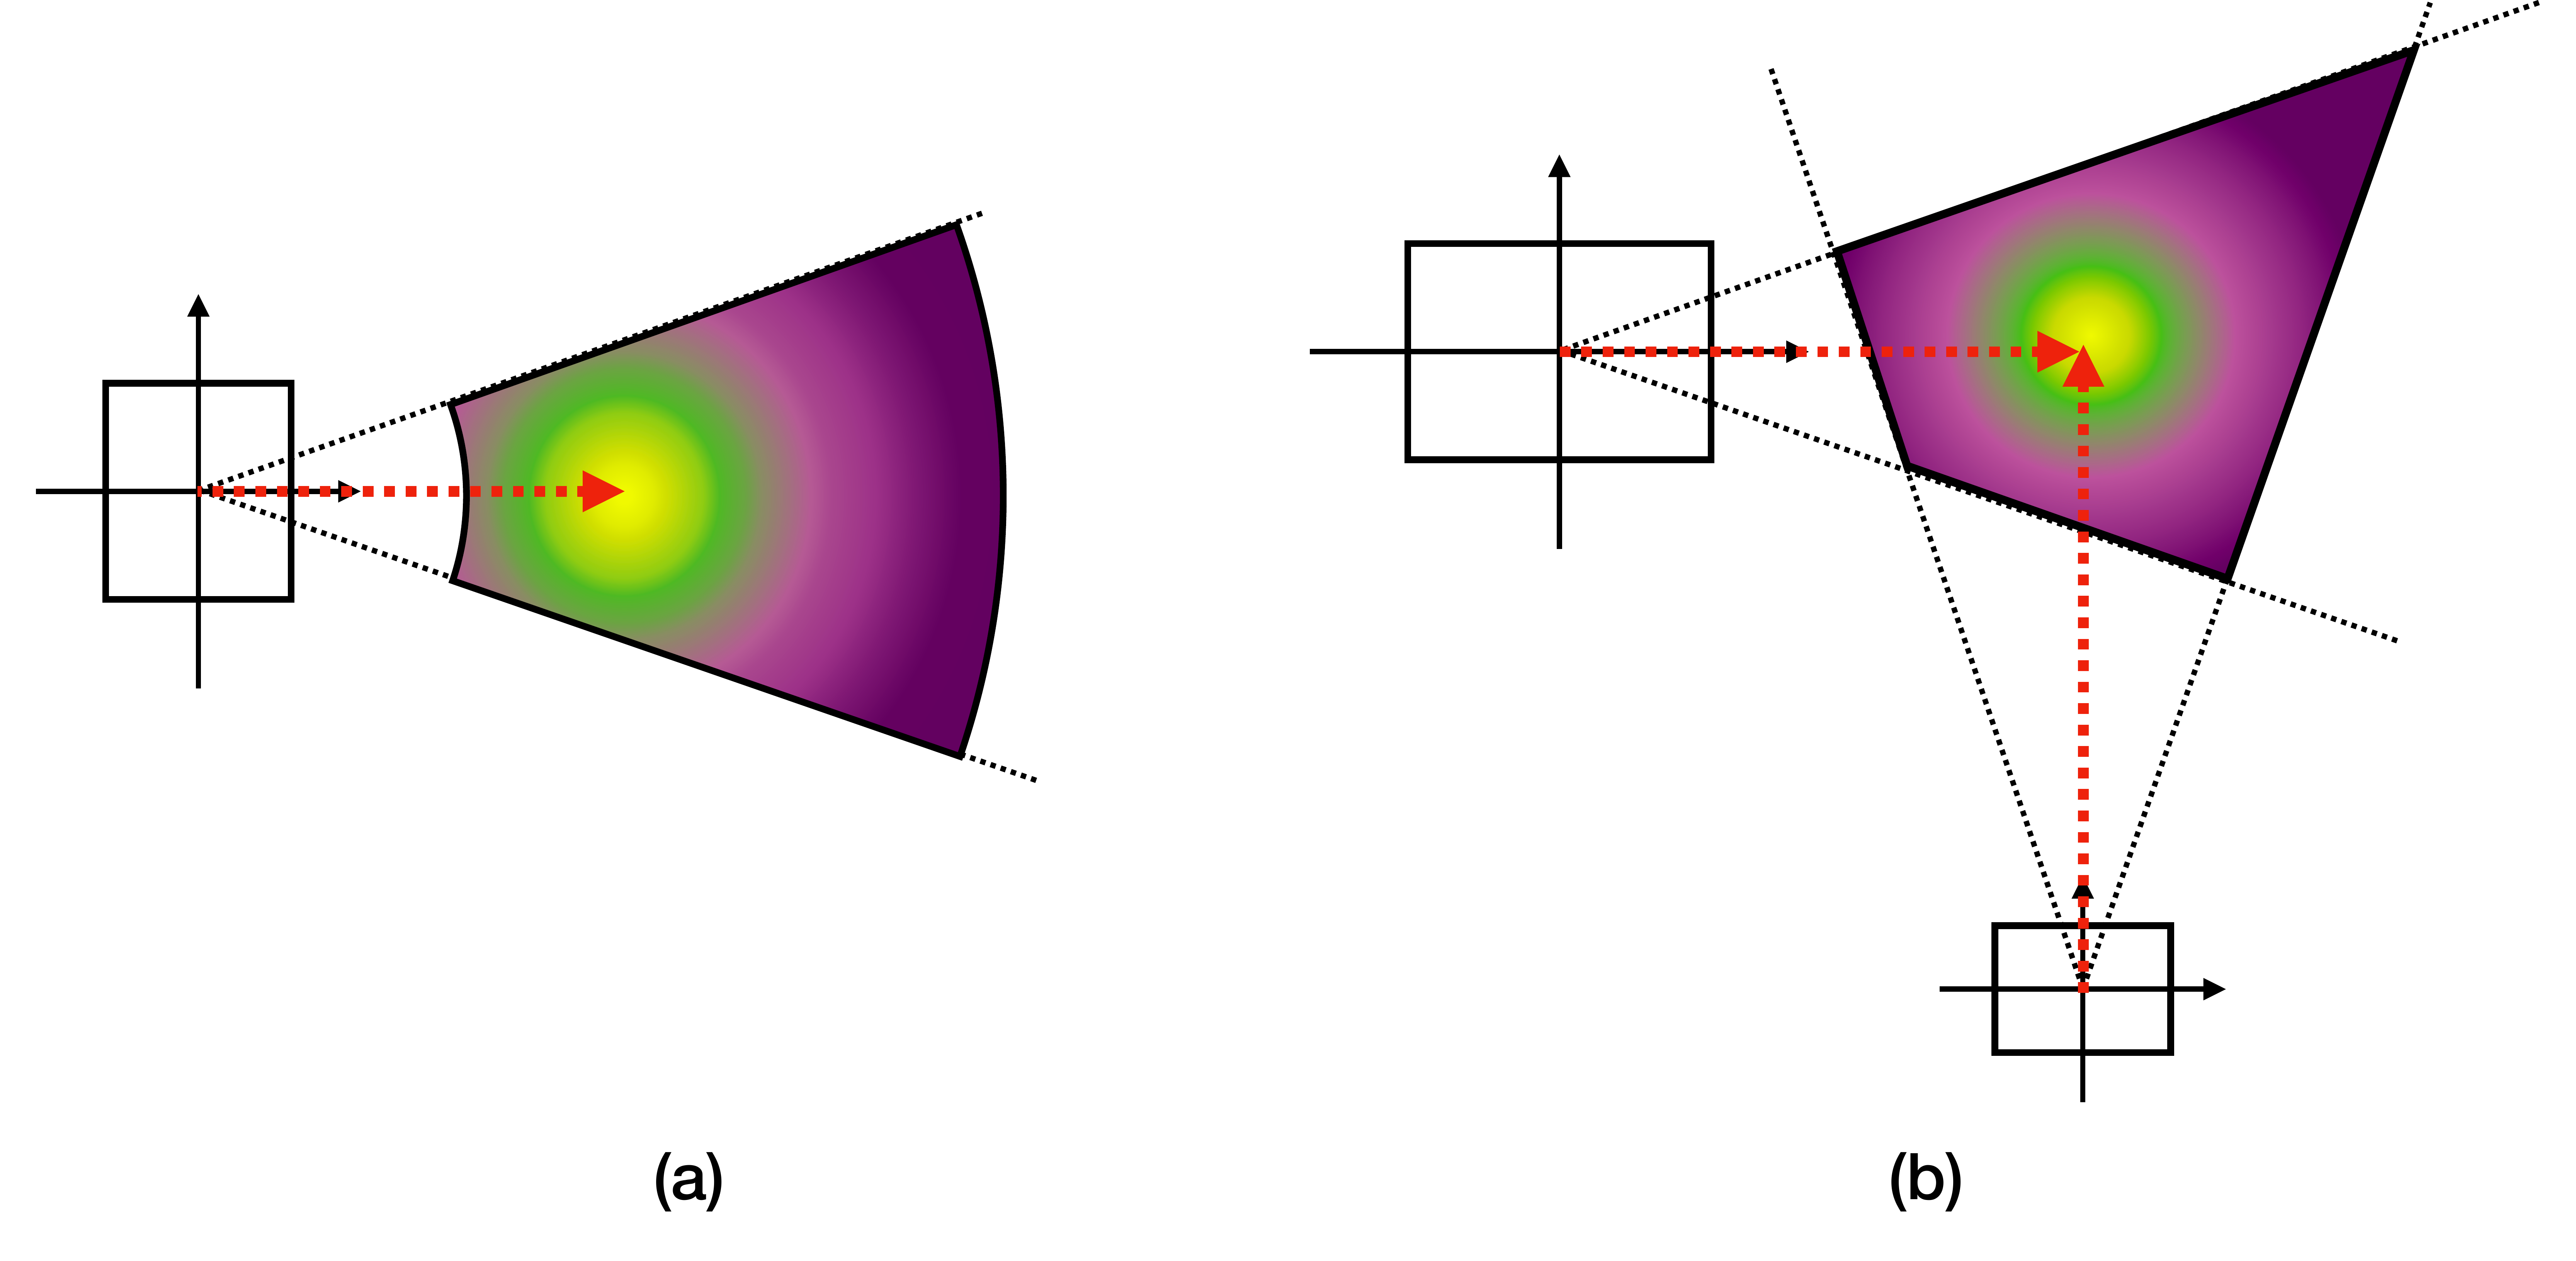}
  \caption{Expert demonstration generation. The demonstration is sampled from a truncated Gaussian distribution. Case (a) illustrates a distribution of ``left-hand side'', where the highlighted area indicates a high probability. We truncate areas that derive from the left side and are too close to the reference object. Case (b) illustrates the composition of spatial relations ``left-hand side'' and ``upper side'', where the conjunction of both directions truncates the distribution. }
  \label{app:fig_gt}
\end{figure}

\begin{figure*}
    \centering
    \includegraphics[width=\textwidth]{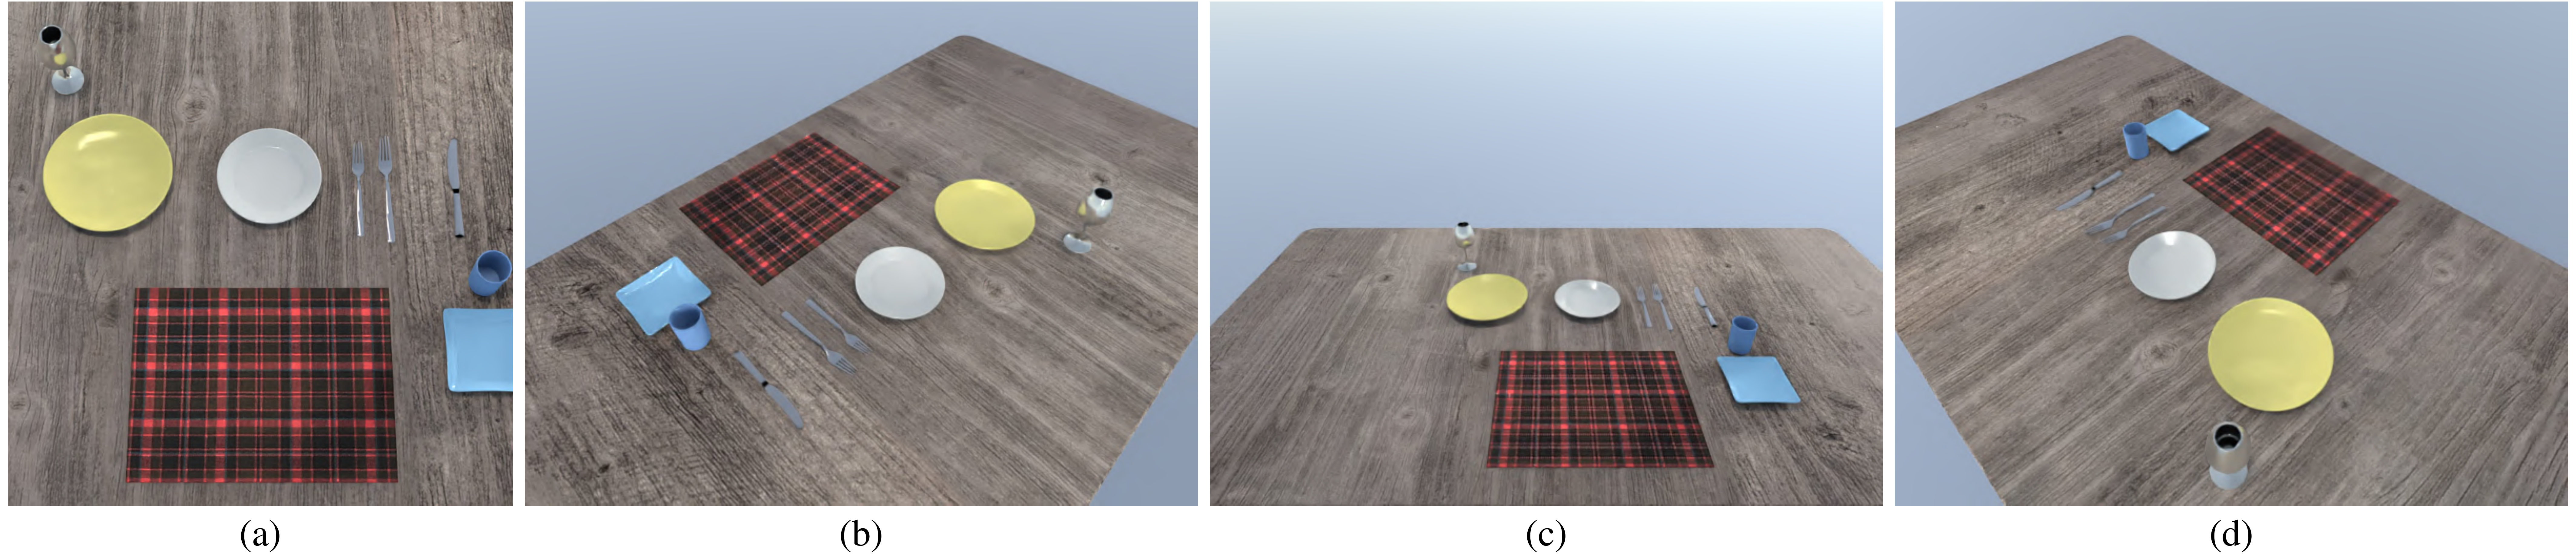}
    \caption{Raw observations captured by cameras in Tabletop Dataset.}
    \label{app:fig_camera}
\end{figure*}

% \begin{figure*}
%     \centering
%     \includegraphics[width=\textwidth]{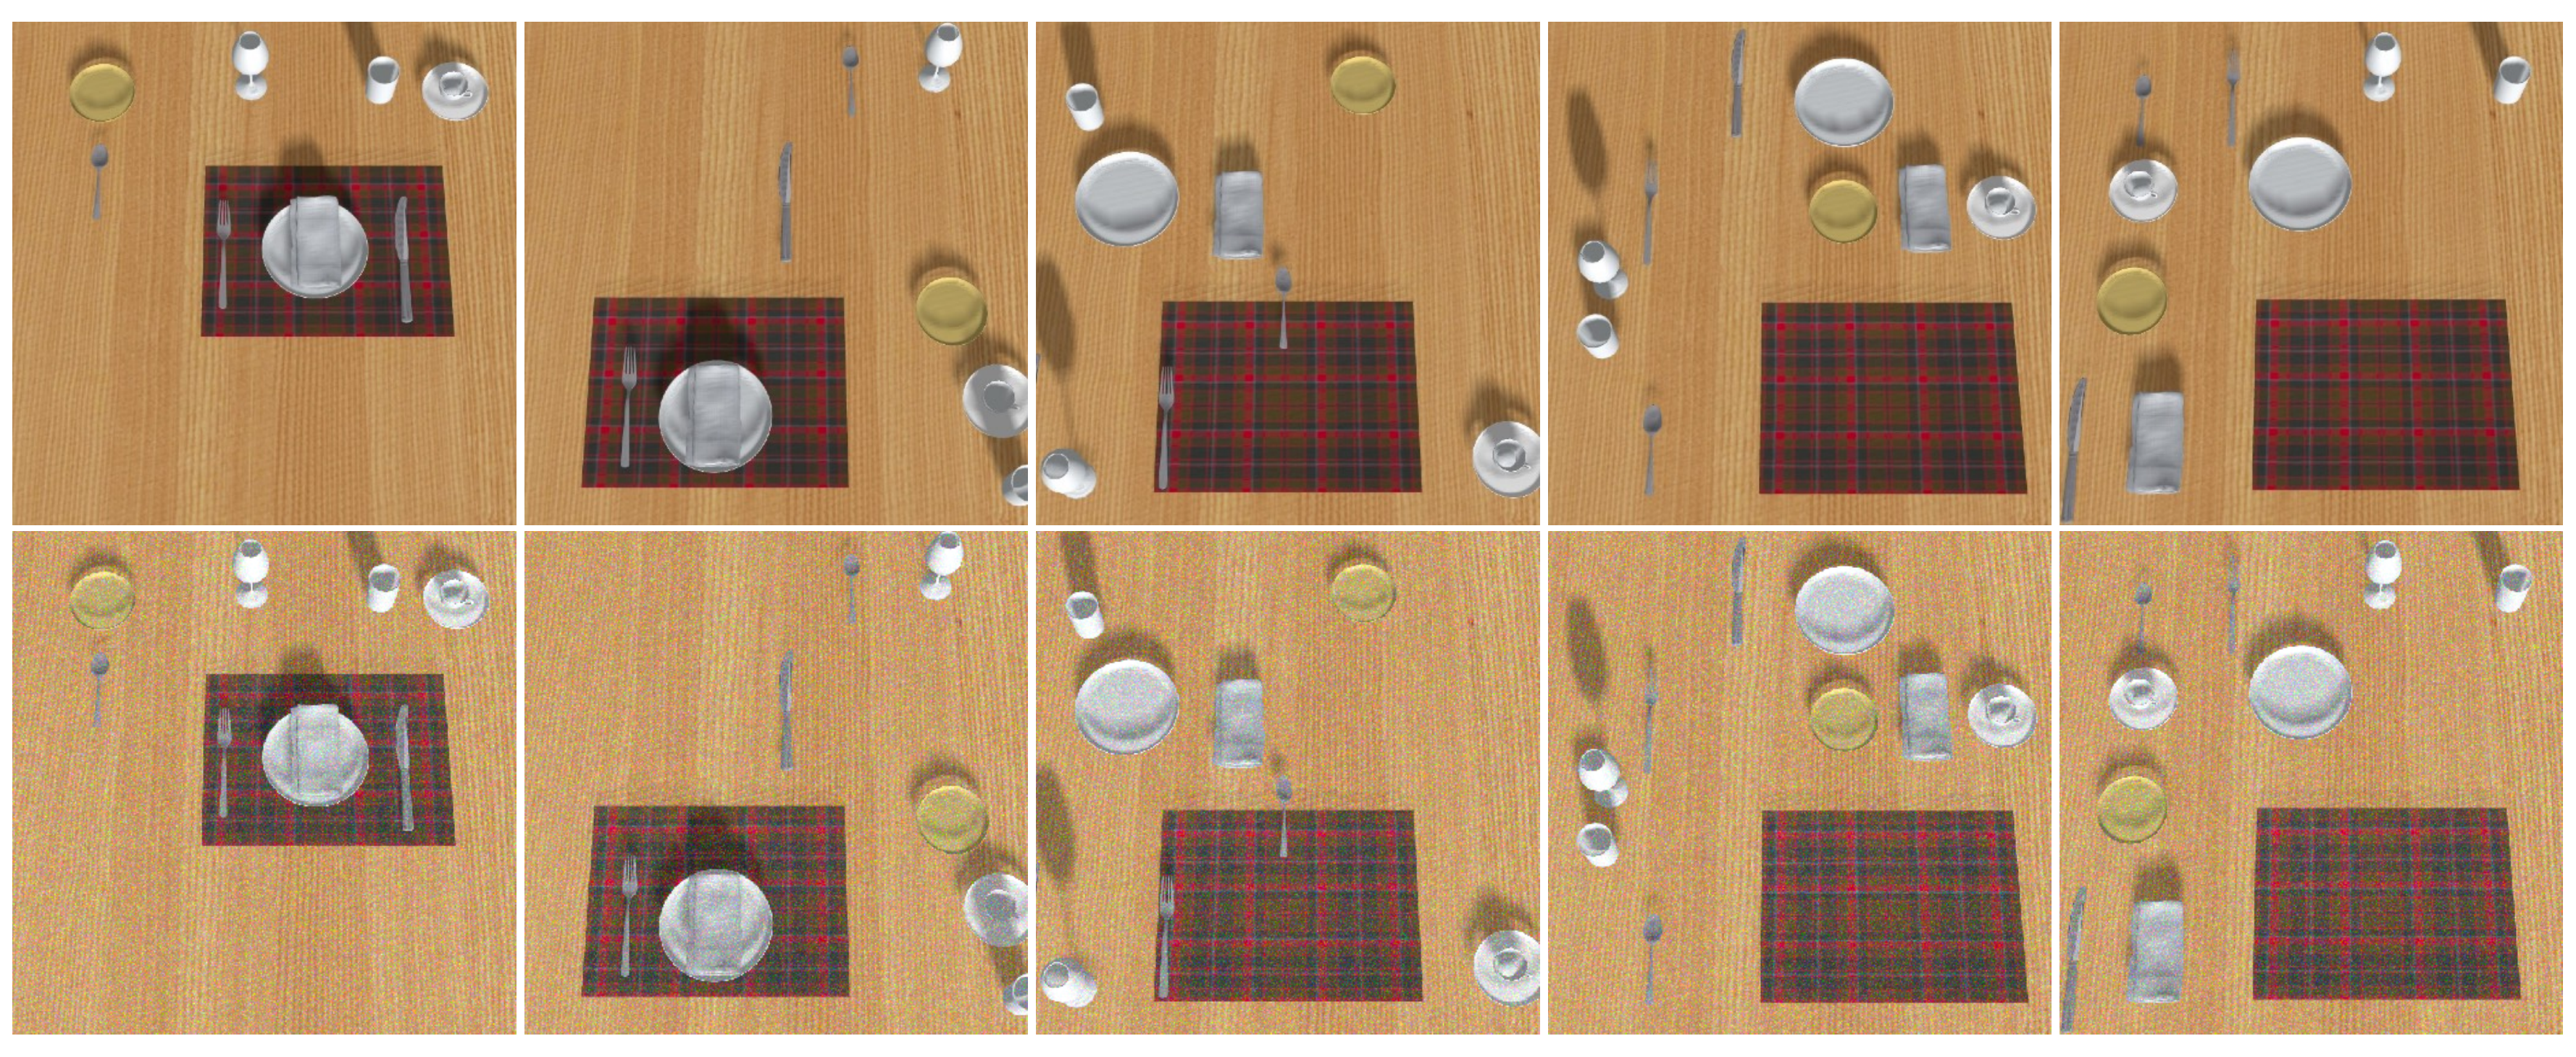}
%     \caption{Demonstration of noisy observation. Raw observations are shown in the top row of images, while noisy observations are shown in the bottom row.}
%     \label{app:fig_noise}
% \end{figure*}

\subsubsection{Expert Demonstration.} We provide a handcrafted policy for expert demonstration in placement generation. According to the ground truth position of objects in the simulator, we sample from a handcrafted Gaussian distribution with a specific direction as the placement generation policy. Specifically, the demonstration is sampled from a truncated Gaussian distribution. There are two examples shown in Fig. 8. In this figure, case (a) illustrates a distribution of ``left-hand side'', where the highlighted area indicates a high probability of placement. We truncate areas that derive from the left side and are too close to the reference object. Case (b) illustrates the composition of spatial relations ``left-hand side'' and ``upper side'', where the conjunction of both directions truncates the distribution. The mean of the Gaussian distribution is located at the intersection of the central axes of the spatial relations.
We also use axis-aligned bounding boxes (AABB) of the target object and context objects to detect intersections and avoid object collision after generating the placement.

\subsection{Evaluation Critera}

We evaluate the success rate of the object placing by examining whether the placement satisfies the spatial relational constraints in the natural language instructions. Specifically, we assess whether the generated particle is located at the truncated regions. For CLIPort, we take the $\mathrm{argmax}$ to get the generated placement. As ParaGon generates a set of particles as the samples of a placement distribution, we randomly sample from the particles ten times to evaluate the success rate.

% \subsection{Task Examples}

% We provide examples of tasks in Table \ref{app:tab_eg}, consisting of raw visual observations (clean), instructions with single and compositional spatial relations and expert demonstrations. 

% Please add the following required packages to your document preamble:
% \usepackage{booktabs}
% \begin{table*}[]
% \centering
% \begin{tabular}{>{\centering\arraybackslash}m{35mm}>{\centering\arraybackslash}m{50mm}>{\centering\arraybackslash}m{50mm}}
% \toprule
%  & Single Spatial Relation & Compositional Spatial Relation \\\midrule
% Raw Observation & \includegraphics[width=0.3\textwidth]{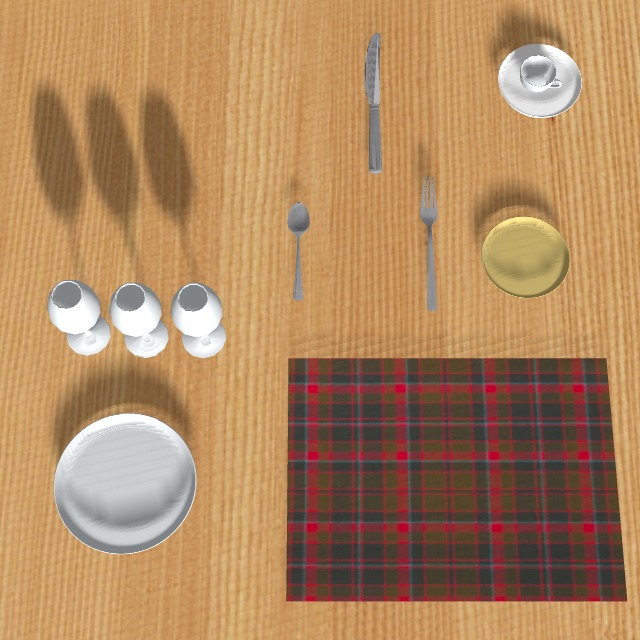} & \includegraphics[width=0.3\textwidth]{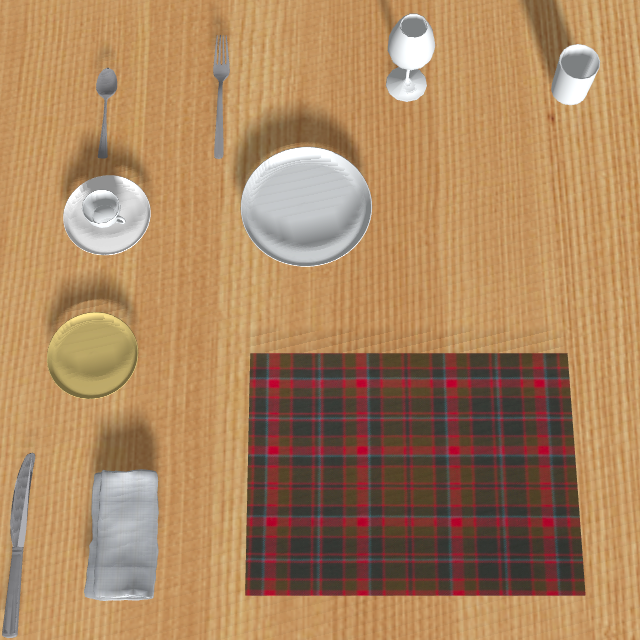} \\ \midrule
% Language Instruction & ``put the wine glass to the left side of the coffee plate.'' & ``put the fork to the left of the water cup and to the right hand side of the wine glass.'' \\ \midrule
% Handcrafted ground-truth distribution & \includegraphics[width=0.3\textwidth]{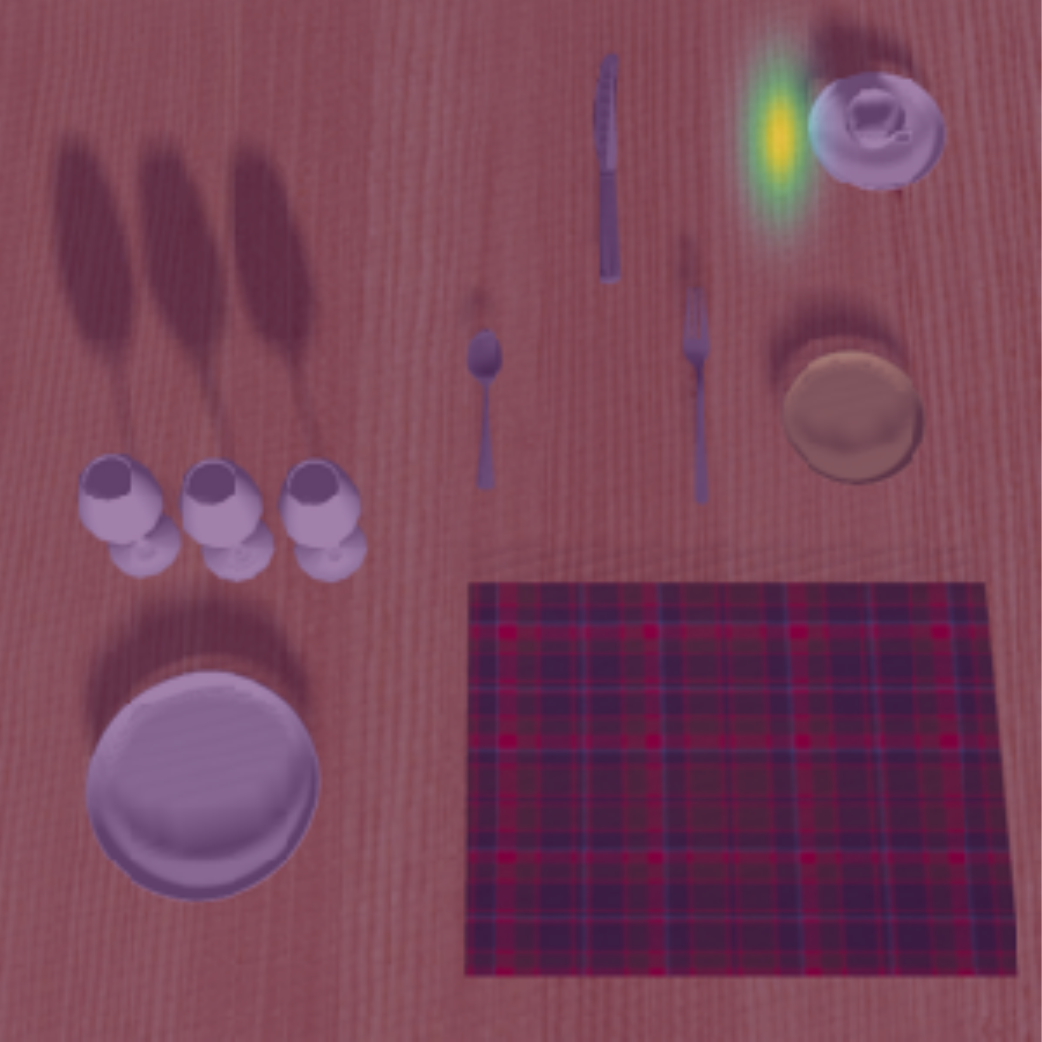} & \includegraphics[width=0.3\textwidth]{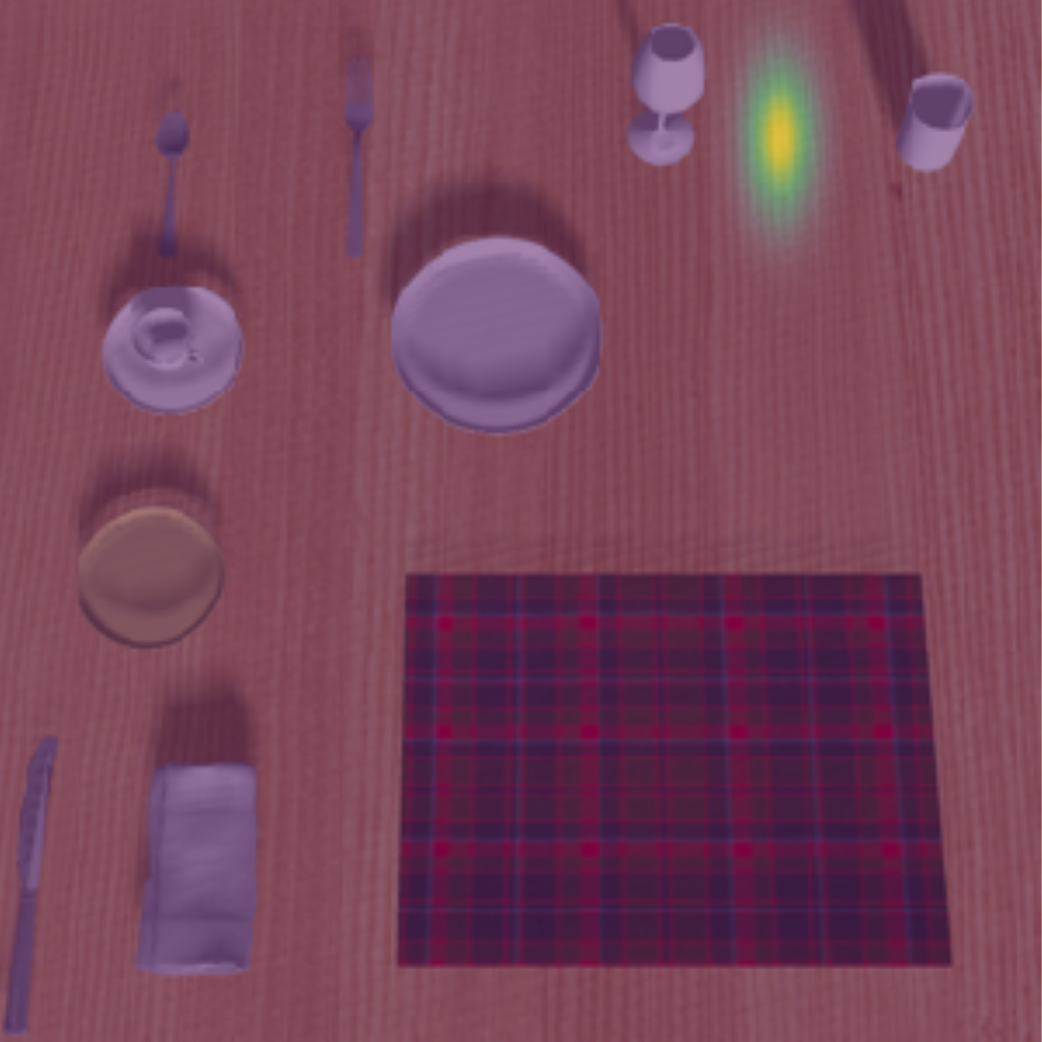} \\\midrule
% Expert Demonstration & \includegraphics[width=0.3\textwidth]{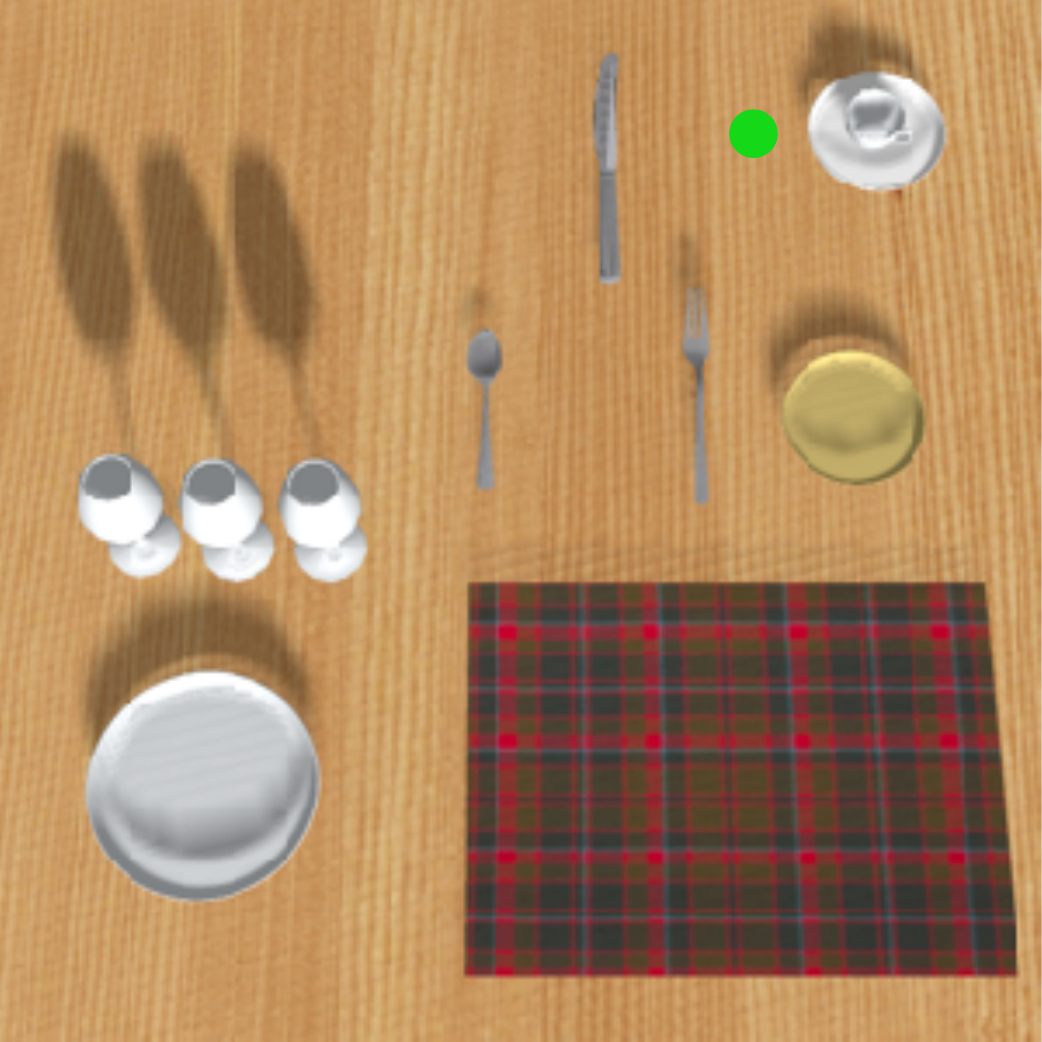} & \includegraphics[width=0.3\textwidth]{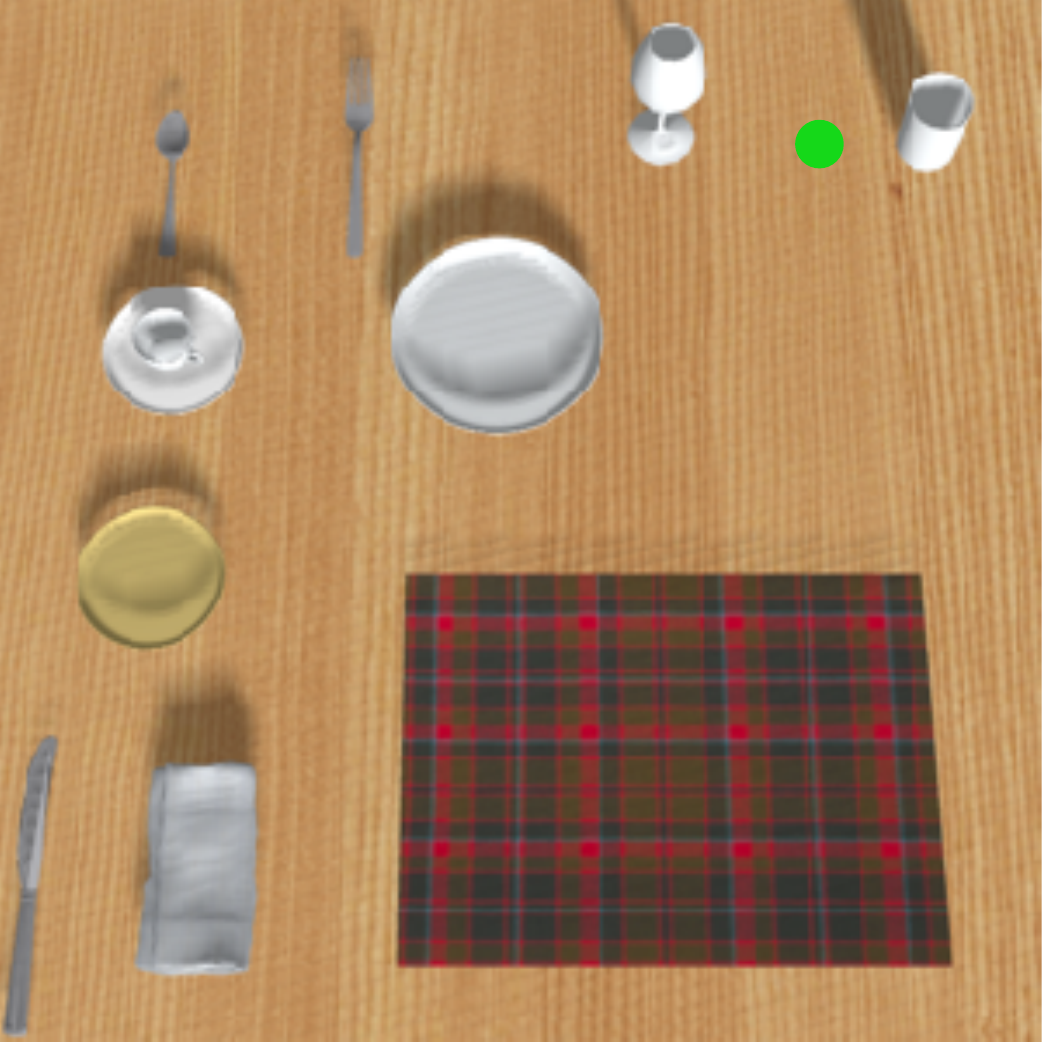} \\ \bottomrule
% \end{tabular}
% \caption{The examples of tasks in Tabletop Dataset.}
% \label{app:tab_eg}
% \end{table*}

% \newpage
\section{Implementation and Training Details}
\label{app:implementation}

% This section introduces the implementation details of \textsc{ParaGon}.

\begin{algorithm}
  \caption{Soft Parsing}
    \begin{algorithmic}[1]
      \INPUT Instruction $\ell=\{\omega_l\}_{l=1}^L$, Text encoder $f_\text{CLIP}(\cdot):\omega \rightarrow \mathbb{R}^{D_\text{word}}$, $K$
      \OUTPUT Triplets: $\{(\varphi_\text{subj}, \varphi_\text{obj}^{(n)}, \varphi_\text{rel}^{(n)})\}_{n=1}^N$, Recovered instruction: $\tilde{\ell}$ 
      \STATE $\tau\leftarrow\text{DepParser}(\ell)$
      \STATE $\{\hbar_l\}_{l=1}^L\leftarrow\text{GNN}(\tau)$
      \STATE $\{a_{\text{subj},l}\}_{l\leq L}\leftarrow\text{SoftMax}(\text{MLP}(\{\hbar_l\}_{l=1}^L))$
      \STATE $\{a^{n}_{\text{obj},l}\}_{n\leq N, l\leq L}\leftarrow \text{SlotAttn}(\{\hbar_l\}_{l=1}^L)$
      \STATE $\hbar^n_\text{obj}\leftarrow\sum_l a^n_{\text{obj},l}\hbar_l$
      \STATE $\{a^{n}_{\text{obj},l}\}_{n\leq N, l\leq L}\leftarrow\text{MHAttn}(\{\hbar^{n}_\text{obj}\}_{n=1}^N, \{\hbar_l\}_{l=1}^L, \{\hbar_l\}_{l=1}^L)$
      \STATE $\varphi_\text{subj}\leftarrow \sum_l a_{\text{subj},l}f_\text{CLIP}(\omega_l)$
      \STATE $\varphi^n_\gamma\leftarrow \sum_l a^n_{\gamma,l}f_\text{CLIP}(\omega_l), \gamma\in\{\text{obj}, \text{rel}\}$ 
      \STATE $\tilde{\varphi}_l=\sum_{n=1}^N\sum_{i\in\{\text{rel}, \text{obj}\}} a_{i,l}^n\varphi^n_i+a_{\text{subj}, l}\varphi_\text{subj}$.
      \STATE $\tilde{\ell}=\text{LSTM}(\{\tilde{\varphi}_l\}_{l=1}^L)$
    \end{algorithmic}
   \label{app:alg_soft_par}
  \end{algorithm}

\subsection{Soft Parsing}
We illustrate the implementation details of the soft parsing module. The algorithm is shown in Algorithm~\ref{app:alg_par_gnn}.

\subsubsection{Structural Prior from Dependency Parsing} We use spaCy dependency parser with transformer backend to get the dependency tree of a given sentence. We use embeddings $v\in\mathbb{R}^{D_\text{embed}}$ to represent the part-of-speech (POS) tag and dependency (DEP) tag in the dependency tree. The message passing neural network uses MLP as the functions $f_m: \mathbb{R}^{D_\text{embed}}\times\mathbb{R}^{D_\text{embed}}\times\mathbb{R}^{D_\text{embed}}\rightarrow\mathbb{R}^{D_\text{embed}}$ and $f_u: \mathbb{R}^{D_\text{embed}}\times\mathbb{R}^{D_\text{embed}}\rightarrow\mathbb{R}^{D_\text{embed}}$. The POS tags are used as the initial node features and the DEP tags are the edge attributes. During the message passing, the node features and edge attributes are concatenated as the input of $f_m$ and $f_u$. Thus, the structural prior from the dependency tree is encoded in the output structural features of the message-passing neural network. In addition, the structure lacks the order of position of the tokens in the sentence. We use cosine positional encoding added in the output structural embeddings to encode the position of tokens in the sentence. 

\subsubsection{Relation Extraction} The output structural features $\hbar_l$ from the message-passing neural network are used for relation extraction. We use attention to evaluate the normalized score of each token in the sentence from message passing for its contribution to the components in relational triplets. We use a single-layer MLP with softmax to compute the normalized score of each token contributing to the subject phrase. To discover potential object phrases, we use slot attention~\cite{locatello2020object} from visual object discovery for unsupervised object phrase discovery. The slot attention algorithm is illustrated in Algorithm \ref{app:alg_slot_attn}. After discovering the object phrases, we use a multi-head attention module to evaluate the relational phrases conditioned on the corresponding object phrases. The object structure embeddings from slot attention are used as the query, and the structural features from message passing as the key and value. After we compute the weights of each token in the sentence for the subject phrase, object phrase, and relational phrase, we use the expected embedding to represent the word embeddings for the phrases in triplets. We use CLIP as the encoder to compute the word embeddings of tokens in the sentence.     

\subsubsection{Hyper-parameters} The dimension of embedding is $D_\text{embed}=64$, and the layer number of message passing neural network is 4. We use 3 iteration for slot attention, with slot number $N_\text{slot}=4$, hidden dimension $D_\text{slots}=128$ and $\epsilon=1\times10^{-8}$. As for the multi-head attention module for relational phrase discovery, the number of heads is eight, and the embedding dimension is 64. Language encoder $\phi(\cdot)$ is trained CLIP (ViT-32/B), in which the word embedding dimension is $D_\text{word}=512$.

\begin{algorithm}
\caption{Slot Attention}
  \begin{algorithmic}[1]
    \INPUT $\text{inputs}\in\mathbb{R}^{N\times D_\text{inputs}}, \text{slots}\sim\mathcal{N}(\mu, \text{diag}(\sigma))\in\mathbb{R}^{K\times D_\text{slots}}$
    \PARAM $k, q, v:$ linear projections for attention; $\text{GRU}$; $\text{MLP}$; $\text{LayerNorm}(\times 3)$
    \STATE $\text{inputs}\leftarrow\text{LayerNorm}(\text{inputs})$
    \FOR{$t=0, \ldots, T$}
        \STATE $\text{slots\_prev} \leftarrow \text{slots}$
        \STATE $\text{slots} \leftarrow \text{LayerNorm} (\text{slots})$
        \STATE $\text{attn}\leftarrow\text{SoftMax}(\frac{1}{\sqrt{D}}k(\text{inputs}) q(\text{slots})^\top, \text{axis}=\text{slots})$
        \STATE $\text{Updates}\leftarrow \text{WeightedMean}(\text{weights}=\text{attn} + \epsilon, \text{values}=v(\text{inputs}))$
        \STATE $\text{slots}\leftarrow \text{GRU} (\text{state}=\text{slots\_prev}, \text{inputs}=\text{updates})$
        \STATE $\text{slots} \leftarrow \text{slots} +  \text{MLP} (\text{LayerNorm} (\text{slots}))$ 
    \ENDFOR
    \OUTPUT $\text{slots}$
  \end{algorithmic}
 \label{app:alg_slot_attn}
\end{algorithm}

\subsection{Particle Mean-field GNN}

The pseudo-code of particle mean-field GNN is illustrated in Algorithm \ref{app:alg_par_gnn}. 

\subsubsection{Functions in Particle Mean-field GNN} For the observation, we use masks of bounding boxes to represent the object positions and shapes in the observed image. We use a simple CNN model $f_\text{pos}:\mathbb{R}^{W_\text{pos}\times H_\text{pos}} \rightarrow \mathbb{R}^{D_\text{pmpnn}}$ to encode the positional feature of the bounding boxes detected in the scene. We then use an MLP to project the positional feature into embeddings. The particle proposal network $f_\psi:\mathbb{R}^{D_\text{pmpnn}}\times \mathbb{R}^{D_\text{pmpnn}} \rightarrow \mathbb{R}^{D_\text{pmpnn}}$ and aggregation network $f_u:\mathbb{R}^{D_\text{pmpnn}} \rightarrow \mathbb{R}^{D_\text{pmpnn}}$ are all single-layer MLP. The reweighting function of observation model $g_\phi:\mathbb{R}^{D_\text{pmpnn}}\times \mathbb{R}^{D_\text{pmpnn}} \rightarrow \mathbb{R}$ is also a MLP. 

\subsubsection{Hyper-parameters}The layer number of particle-based mean-field GNN is $T=8$. In message passing, we use embeddings with dimension $D_\text{pmpnn}=128$. In soft resampling, we use $\alpha = 0.5$ for training and $\alpha=1.0$ for inference. For visual grounding, the visual encoder is pre-trained CLIP (ViT-32/B).

\begin{algorithm}[]
\caption{Particle Mean-field GNN}
  \begin{algorithmic}[1]
    \INPUT Number of layer $T$, number of particles $K$, detected object bounding boxes $\mathbf{B}=\{(\obs_m, \bfx_m)\}_{m=1}^M$, relational graph $\mathcal{G}=(\mathcal{V}, \mathcal{E})$, edge attributes (spatial relation embeddings) $r_{ij}$
    \STATE ${h}_{i,k}^{(0)}\sim\mathcal{N}(0, 1),~w_{i,k}^{(0)}\leftarrow 1/K,~t\leftarrow 0$\hfill\COMMENT{Initialization}
    \FOR{$t<T$}
        \FOR{$(i,j)\in\mathcal{E}$}\hfill\COMMENT{Message Computing}
            \STATE $m_{ji,k}^t=f_\psi(h_{j,k}^{t-1}, r_{ij})$
            \STATE $m_{\text{obs},j}^t= f_\phi (\sum_{m=1}^Mb_m^jf_\text{pos}(\bfy_m))$
            \STATE $w_{ji, k}^t=\eta w_{j,k}^{t-1}\log g_\phi(h_{j,k}^{t-1}, m^t_{\text{obs},j})$
        \ENDFOR
        \FOR{$i\in\mathcal{V}$}\hfill\COMMENT{Message Aggregation}
            \STATE $h_{i,k}^t=f_u(\sum_{j\in N(i)}m_{ji, k}^t + m_{\text{obs},i}^t)$
            \STATE $\log w_{i,k}^t=c + \log g_\phi(h_{i,k}^{t}, m^t_{\text{obs}, i}) + \sum_{j\in N(i)} w_{ji,k}^{t}$
            \STATE $\{(h'^t_{i,k}, w'^t_{i,k})\}_{k=1}^K=\text{SoftResamp}(\{(h^t_{i,k}, w^t_{i,k})\}_{k=1}^K)$
        \ENDFOR
        \STATE $t \leftarrow t + 1$
    \ENDFOR
    \STATE $x^*_{i,k}=\pi_\text{dec}(h'^T_{i,k}), \forall k\leq K$ \hfill\COMMENT{Decode Placement}
    \OUTPUT $\{(x^*_{i,k}, w'^T_{i,k})\}_{k=1}^K$ 
  \end{algorithmic}
  \label{app:alg_par_gnn}
\end{algorithm}

\subsection{Training}

We conduct supervised learning to train the model end-to-end. There are two components to the training objective. One is the negative log-likelihood of dataset $\bar{\mathcal{X}}$: $\mathcal{J}_l=\sum_{\bar{\bfx}\in\bar{\mathcal{X}}}-\log \sum_{k} w^*_k\mathcal{N}(\bar{\bfx};\mathbf{x}^*_{k}, \Sigma)$, where $\bar{\bfx}\in\bar{\mathcal{X}}$ is the labeled placement and the likelihood is a mixture of Gaussian represented by each output particle of target object $\{(\mathbf{x}^*_k, w^*_k)\}_{k=1}^K$. We also minimize the auxiliary loss for improving soft parsing: $\mathcal{J}_s=\sum_{\ell\in\bar{\mathcal{X}}}||\ell - \tilde{\ell}||^2=\sum_{\ell\in\bar{\mathcal{X}}}\sum_l (\omega_l - \tilde{\omega}_l)^2$. As such, the final objective is: $\mathcal{J}=\mathcal{J}_l + \lambda\mathcal{J}_s$, where $\lambda$ is a hyper-parameter. The hyper-parameter $\lambda=10.0$. For target object grounding, we use cross-entropy loss, where the labels for the loss function are the closest bounding box to the ground truth object position. 

For training, we use Adam optimizer, and the learning rate is $1\times 10^{-4}$. We train the model for 200K steps when the data is more significant than 1000 and 50K when trained by 300. 

\subsection{Baseline Implementation}

\subsubsection{No Soft Parsing}

This baseline model directly uses the embedding of the entire instruction sentence instead of the embeddings from triplets for object grounding and message passing in step 4 of Algorithm \ref{app:alg_par_gnn}.

\subsubsection{No Particle}

This baseline model does not have particles in the message passing, and the initially hidden features in step 1 of Algorithm~\ref{app:alg_par_gnn} are vectors with zero values. It also does not have step 11 for soft parsing.

\subsubsection{No Resampling}

The third baseline is built without soft resampling in step 11 of Algorithm \ref{app:alg_par_gnn}.

\subsubsection{\textsc{ParaGon}(ViT + Bert)}

This baseline model uses the ImageNet-pretrained ViT-32/B model for visual encoding and the pretrained Bert model for text encoding in visual grounding, representing the edge attribute $r_{ij}$.
% \begin{figure*}[h]
%     \centering
%     \makebox[\textwidth][c]{
%     \includegraphics[width=1.0\textwidth]{figs/example_pag_simple.pdf}}
%     \caption{Example placements by P\&G}
%     \label{app:fig_pag}
% \end{figure*}

% \begin{figure*}[h]
%     \centering
%     \makebox[\textwidth][c]{
%     \includegraphics[width=1.0\textwidth]{figs/example_p&g.pdf}}
%     \caption{Example placements by P\&G}
%     \label{app:fig_pag_2}
% \end{figure*}

% \begin{figure*}[h]
% \makebox[\textwidth][c]{
%     \centering
%     \includegraphics[width=1.0\textwidth]{figs/cliport_demo.pdf}}
%     \caption{Example placements by CLIPort}
%     \label{app:fig_cliport}
% \end{figure*}
