# Supplementary material for: Differentiable Parsing and Visual Grounding of Natural Language Instructions for Object Placement
Source: arXiv:2210.00215 source file (2023-03-13)
Supplement: Supplementary file 3 [file 7_appendix.tex]

\appendices 

\section{Tabletop Dataset}
\label{app:dataset}

We extend the dataset from \href{https://github.com/AdaCompNUS/table-setting-dataset}{\color{blue}{https://github.com/AdaCompNUS/table-setting-dataset}} with randomly sampled objects and generate placement from several sampled spatial relations. 

\subsection{Objects}

We samples from 19 dinning objects with 8 classes, including forks, knives, spoons, plates, wine glasses, a water cup, a coffee cup, and a napkin cloth. All the objects are described in Figure.

\subsection{Language Expressions}

Our dataset draws samples from commonly used spatial relations with various language expressions. The spatial relations includes left, right, front, behind, on top of, and their compositions. We also have ternary spatial relation ``between''. The language expressions for each spatial relations are illustrated in Table \ref{app:tab_rel}.

% Please add the following required packages to your document preamble:
% \usepackage{booktabs}
% Please add the following required packages to your document preamble:
% \usepackage{booktabs}
\begin{table*}[]
\centering
\begin{tabular}{@{}llll@{}}
\toprule
Spatial Relations &
  Language Expressions &
  Spatial Relations &
  Language Expressions \\ \midrule
Left &
  \begin{tabular}[c]{@{}l@{}}``to the left of''\\ ``to the left side of''\\ ``to the left hand side of''\end{tabular} &
  Front Right &
  \begin{tabular}[c]{@{}l@{}}``to the lower right of''\\ ``to the lower right side of''\\ ``to the lower right corner of''\\ ``to the front right of''\end{tabular} \\ \midrule
Right &
  \begin{tabular}[c]{@{}l@{}}``to the right of''\\ ``to the right side of''\\ ``to the right hand side of''\end{tabular} &
  Behind Left &
  \begin{tabular}[c]{@{}l@{}}``to the upper left of''\\ ``to the upper left side of''\\ ``to the upper left corner of''\end{tabular} \\ \midrule
Front &
  \begin{tabular}[c]{@{}l@{}}``in front of''\\ ``to the lower side of''\end{tabular} &
  Behind Right &
  \begin{tabular}[c]{@{}l@{}}``to the upper right of''\\ ``to the upper right side of''\\ ``to the upper right corner of''\end{tabular} \\ \midrule
Behind &
  \begin{tabular}[c]{@{}l@{}}``behind''\\ ``to the upper side of''\end{tabular} &
  on top of &
  \begin{tabular}[c]{@{}l@{}}``on''\\ ``above''\\ ``on top of''\\ ``on the center of''\end{tabular} \\ \midrule
Front Left &
  \begin{tabular}[c]{@{}l@{}}``to the lower left of''\\ ``to the lower left side of''\\ ``to the lower left corner of''\\ ``to the front left of''\end{tabular} &
   &
   \\ \bottomrule
\end{tabular}
\vspace{3mm}
\caption{Spatial relations and their language expressions in Tabletop Dataset.}
\label{app:tab_rel}
\end{table*}

\subsection{Data Generation}

\subsubsection{Instruction Generation}

We generate the instructions according to language templates. The template for tasks with single spatial relation is illustrated below:
\begin{align}
    &\text{[verb phrase]} + \text{[subject phrase]} \\&+ \text{[spatial relation phrase]} + \text{[object phrase]}.
\end{align}
If the language instruction contains compositional spatial relations, the template is:
\begin{align}
    &\text{[verb phrase]} + \text{[subject phrase]} \\+& \text{[spatial relation phrase 1]} + \text{[object phrase 1]}\\+&\text{``and''}+ \text{[spatial relation prhase 2]} + \text{[object phrase 2]}.
\end{align}
The spatial relations are sampled from the Table \ref{app:tab_rel} and the subject phrases and object phrases are sampled from Table \ref{app:tab_obj}. We sample the verb phrases uniformly as random from ``put'', ``place'', and ``move''.

% Please add the following required packages to your document preamble:
% \usepackage{booktabs}
% \begin{table}[]
% \centering
% \begin{tabular}{P{30mm}P{40mm}}

% \toprule
% Objects      & Language Expressions \\ \midrule
% \begin{tabular}[c]{@{}c@{}}Dinner Fork\\ Salad Fork\\ Dessert Fork\end{tabular}    & ``the fork''  \\ \midrule
% \begin{tabular}[c]{@{}c@{}}Dinner Knife\\ Salad Knife\\ Dessert Knife\end{tabular} & ``the knife'' \\ \midrule
% \begin{tabular}[c]{@{}c@{}}Dinner Spoon\\ Soup Spoon\end{tabular}                  & ``the spoon'' \\ \midrule
% \begin{tabular}[c]{@{}c@{}}Charger\\ Dinner Plate\\ Bread Plate\end{tabular}       & ``the plate'' \\ \midrule
% Coffee Cup   & ``the coffee cup''   \\ \midrule
% Wine Glass   & ``the wine glass''   \\ \midrule
% Water Cup    & ``the water cup''    \\ \midrule
% Napkin Cloth & ``the napkin cloth'' \\ \bottomrule
% \end{tabular}
% \vspace{3mm}
% \caption{The object expressions of Tabletop Dataset.}
% \label{app:tab_obj}
% \end{table}

\begin{table*}[]
\centering
\begin{tabular}{@{}llll@{}}
\toprule
Objects                                                                            & Language Expressions & Objects    & Language Expressions \\ \midrule
\begin{tabular}[l]{@{}l@{}}Dinner Fork\\ Salad Fork\\ Dessert Fork\end{tabular} &
  ``the fork'' &
  \begin{tabular}[l]{@{}l@{}}Charger\\ Dinner Plate\end{tabular} &
  ``the plate'' \\ \midrule
\begin{tabular}[l]{@{}l@{}}Dinner Knife\\ Salad Knife\\ Dessert Knife\end{tabular} & ``the knife''        & Coffee Cup & ``the coffee cup''   \\ \midrule
\begin{tabular}[l]{@{}l@{}}Dinner Spoon\\ Soup Spoon\end{tabular}                  & ``the spoon''        & Wine Glass & ``the wine glass''   \\ \midrule
\begin{tabular}[l]{@{}l@{}} Salad Plate\end{tabular}       & ``the salad plate''        & Water Cup  & ``the water cup''    \\ \midrule
Napkin Cloth                                                                       & ``the napkin cloth'' &            &                      \\ \bottomrule
\end{tabular}
\vspace{3mm}
\caption{The object expressions of Tabletop Dataset}
\label{app:tab_obj}
\end{table*}

\subsubsection{Image Generation}

\textbf{Camera Setup.} We use 4 cameras to capture the visual observation. Similar to the Raven simulator, there are three RGB-D cameras with resolutions of $640\times 480$ that are placed on the rectangular table's top, left, and right, pointing towards the center (see (a), (b), and (c) in Figure \ref{app:fig_camera}). We also have an RGB camera with a resolution of $640\times 640$ placed at the top of the table (see (d) in Figure \ref{app:fig_camera} for the example picture).

\begin{figure*}
    \centering
    \includegraphics[width=\textwidth]{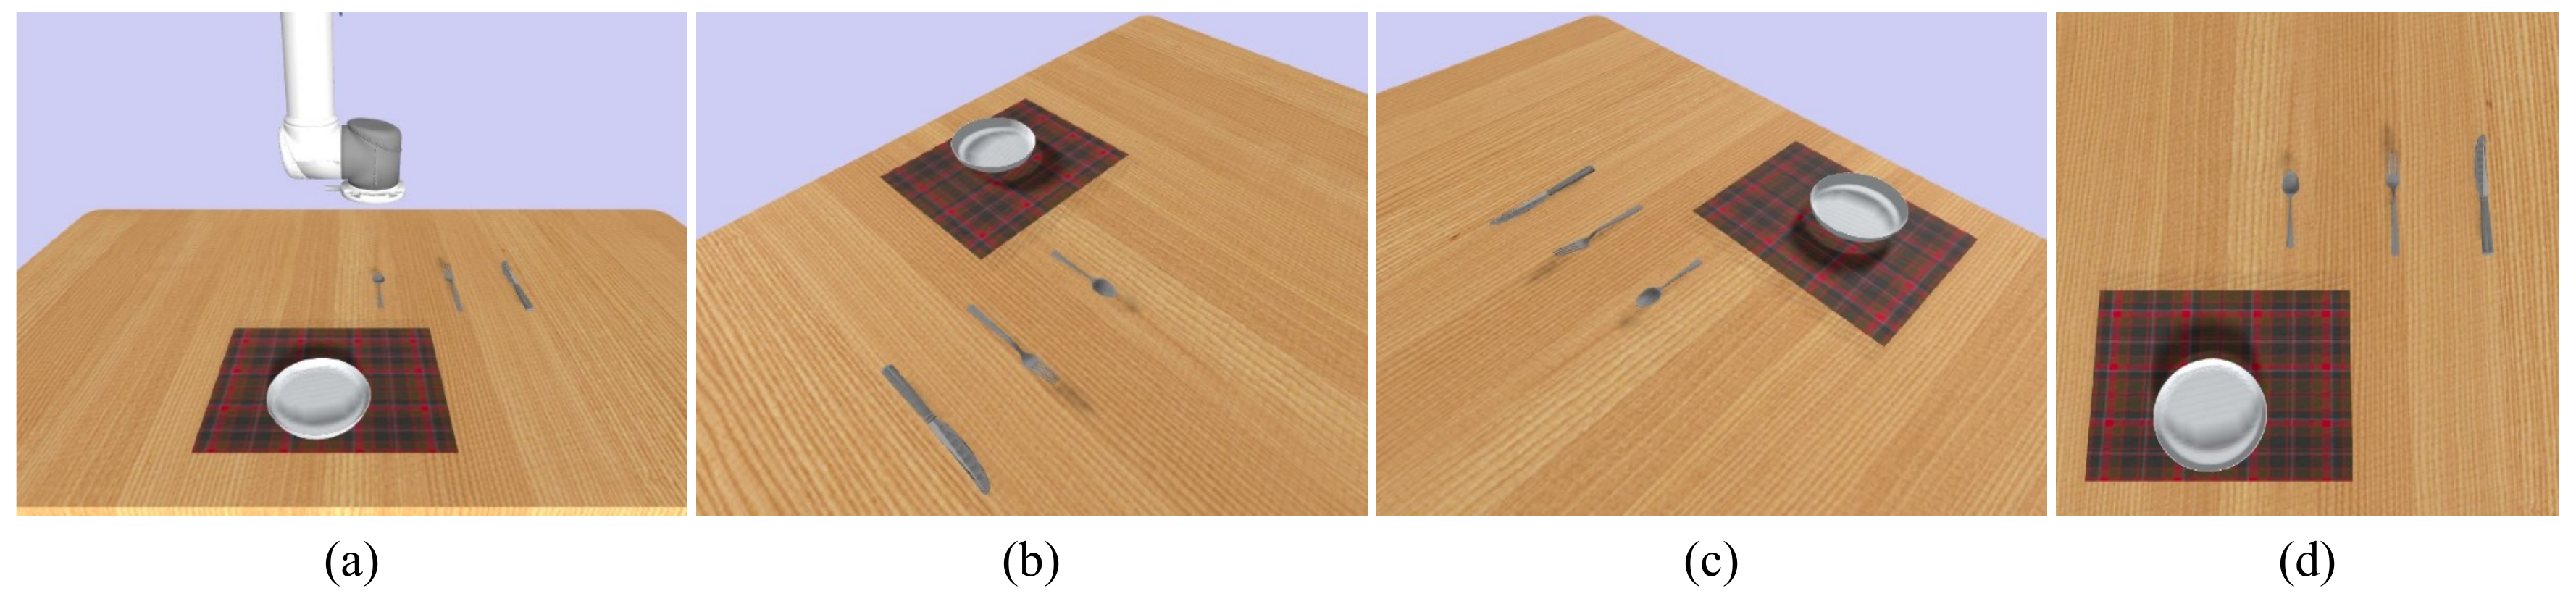}
    \caption{Raw observations captured by cameras in Tabletop Dataset.}
    \label{app:fig_camera}
\end{figure*}

\textbf{Noisy Observation.} In ablation study, we add strong Gaussian noise $\mathcal{N}(0, 10)$ to the image to test the robustness of the methods. See Figure \ref{app:fig_noise} for the example pictures. 

\begin{figure*}
    \centering
    \includegraphics[width=\textwidth]{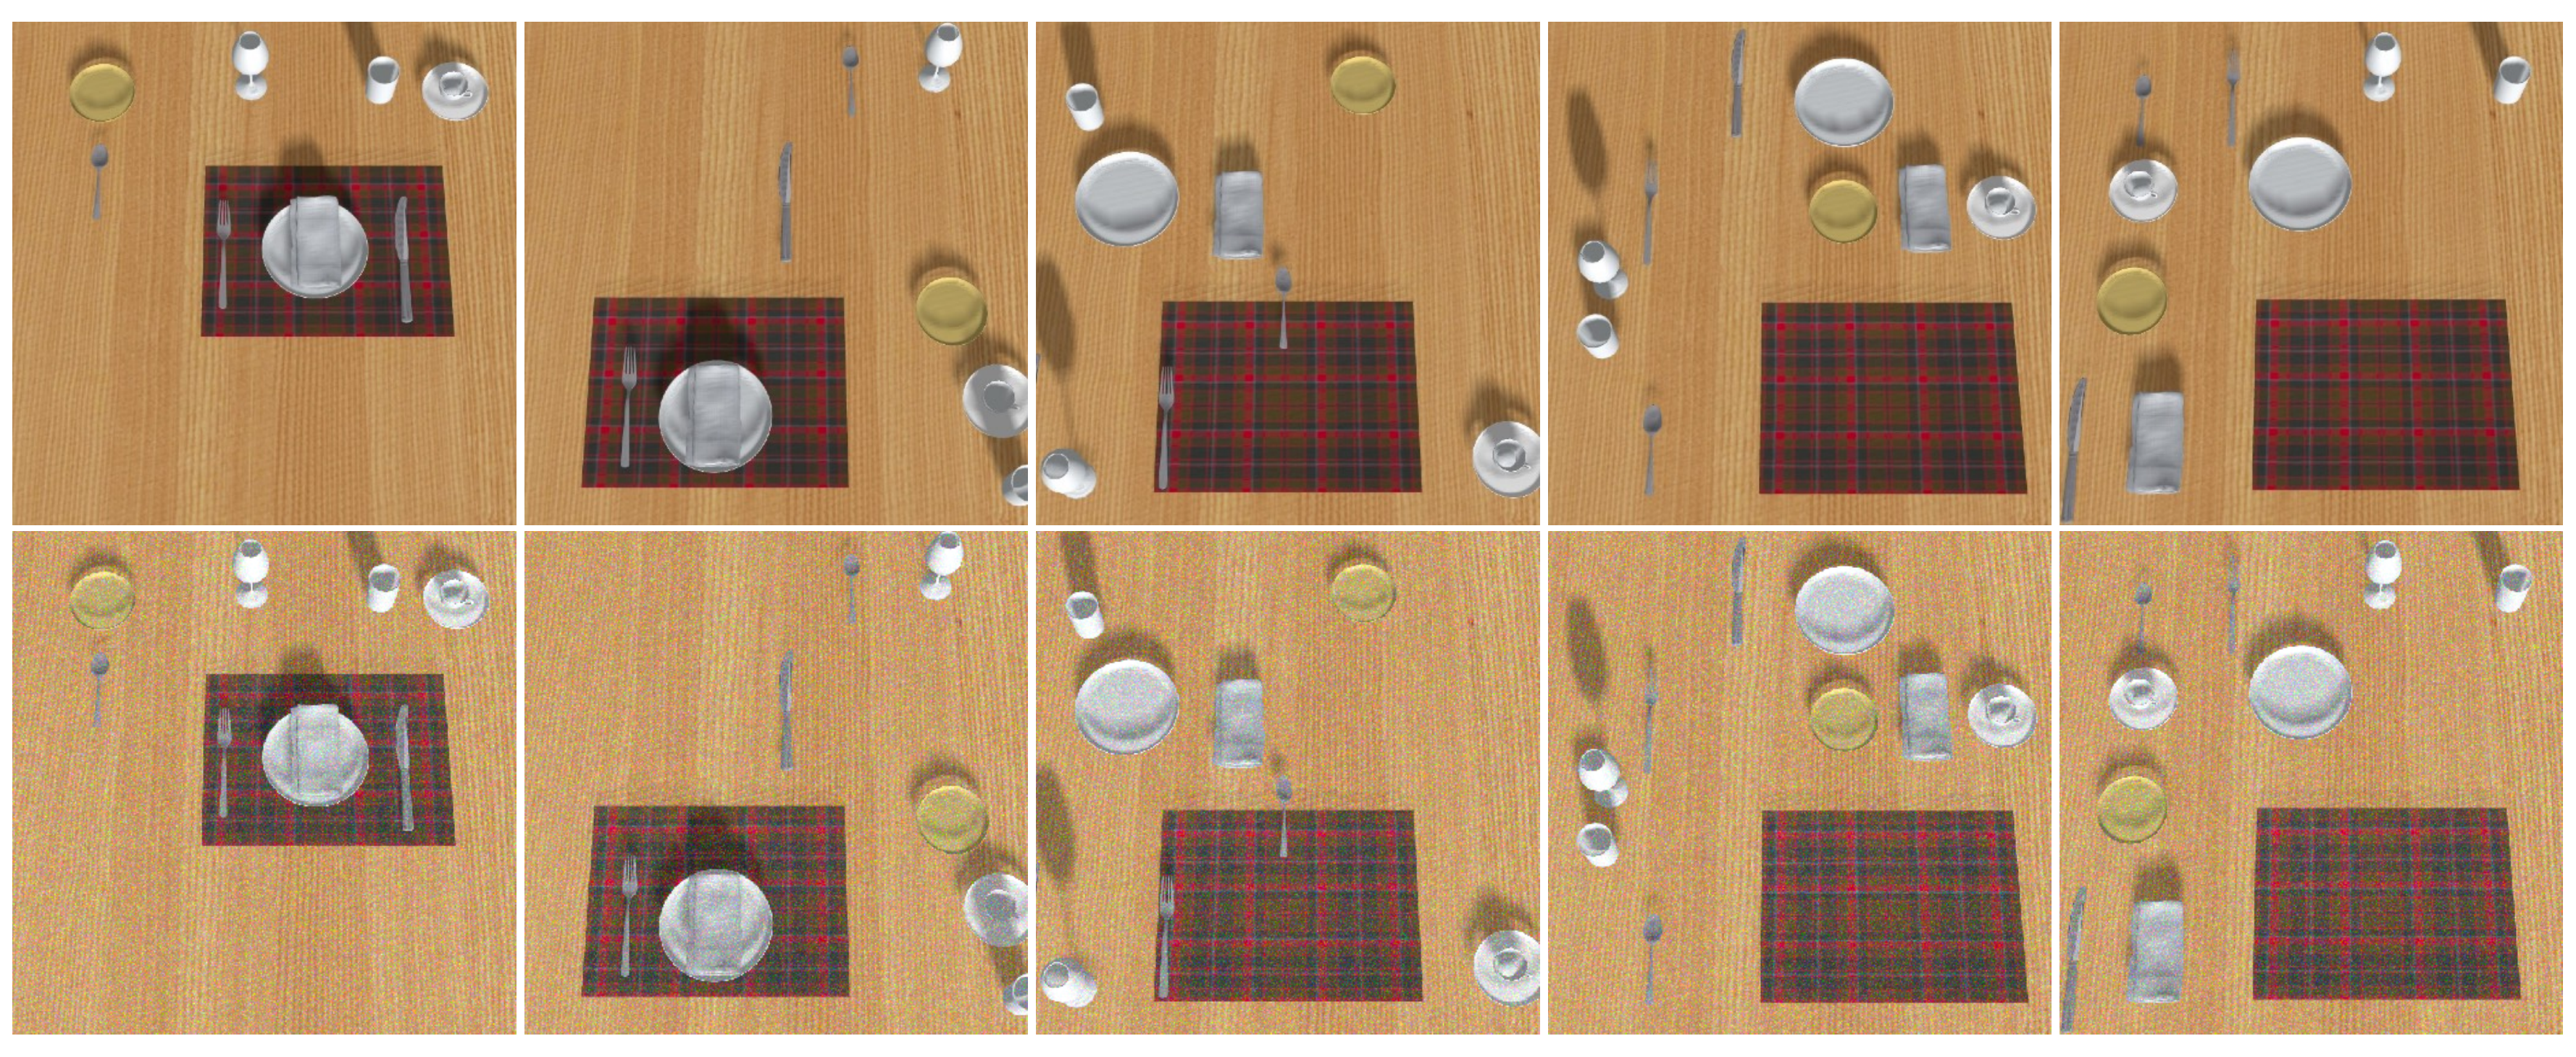}
    \caption{Demonstration of noisy observation. Raw observations are shown in the top row of images, while noisy observations are shown in the bottom row.}
    \label{app:fig_noise}
\end{figure*}

\subsubsection{Expert Demonstration.} We provide a handcrafted policy for expert demonstration in placement generation. According to the groundtruth position of objects in the simulator, we sample from a handcrafted Gaussian distribution with specific direction as the placement generation policy. 
\begin{equation}
    \mathbf{x}_\text{gt} \sim \mathcal{N}(\mathbf{x}_\text{ctx} +d \cdot \mathbf{e}, (\mathbf{I} \mathbf{s}_\text{ctx}^\top)^2)
\end{equation}
For compositional spatial relations, the mean and variance of the distribution is conditioned on the distance between objects. Equation shows the Gaussian distribution. We also use axis-aligned bounding boxes (AABB) of target object and context objects to detect intersection and avoid object collision after generate the placement. Thus, the groundtruth distribution of the object placement in our dataset is a truncated Gaussian distribution or a truncated Gaussian Mixture Model. 

\subsection{Task Examples}

We provide examples of tasks in Table \ref{app:tab_eg}, consisting of raw visual observations (clean), instructions with single and compositional spatial relations and expert demonstrations. 

% Please add the following required packages to your document preamble:
% \usepackage{booktabs}
\begin{table*}[]
\centering
\begin{tabular}{>{\centering\arraybackslash}m{35mm}>{\centering\arraybackslash}m{50mm}>{\centering\arraybackslash}m{50mm}}
\toprule
 & Single Spatial Relation & Compositional Spatial Relation \\\midrule
Raw Observation & \includegraphics[width=0.3\textwidth]{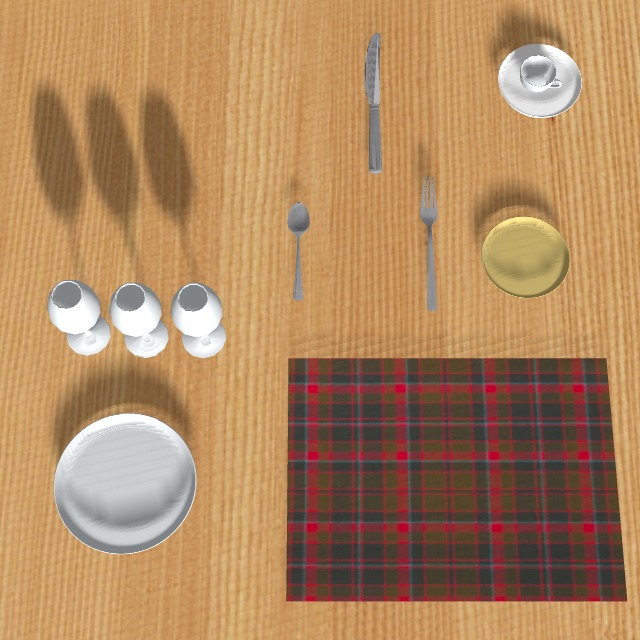} & \includegraphics[width=0.3\textwidth]{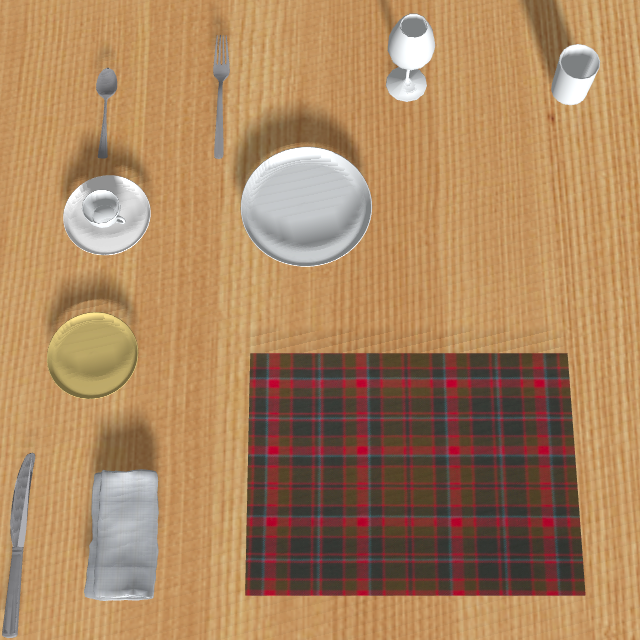} \\ \midrule
Language Instruction & ``put the wine glass to the left side of the coffee plate.'' & ``put the fork to the left of the water cup and to the right hand side of the wine glass.'' \\ \midrule
Handcrafted ground-truth distribution & \includegraphics[width=0.3\textwidth]{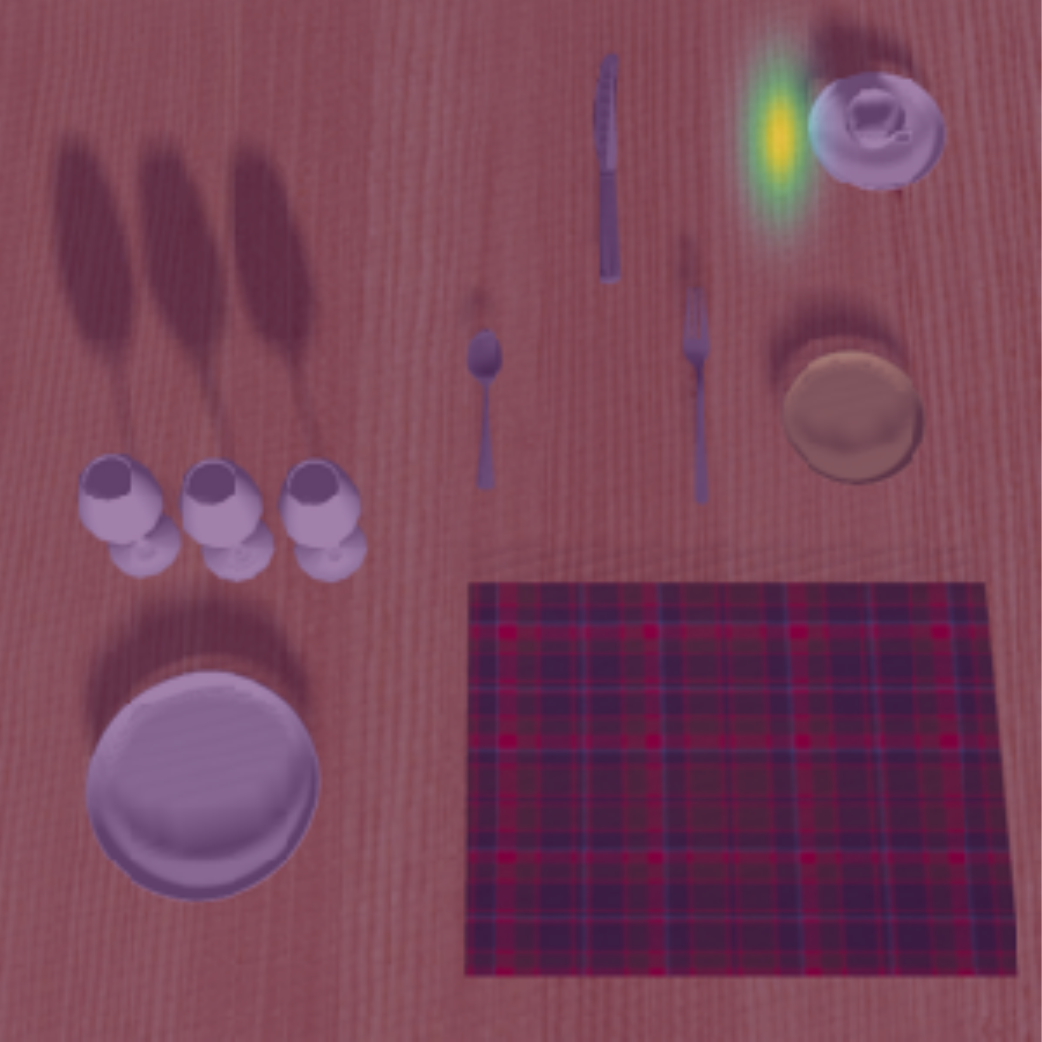} & \includegraphics[width=0.3\textwidth]{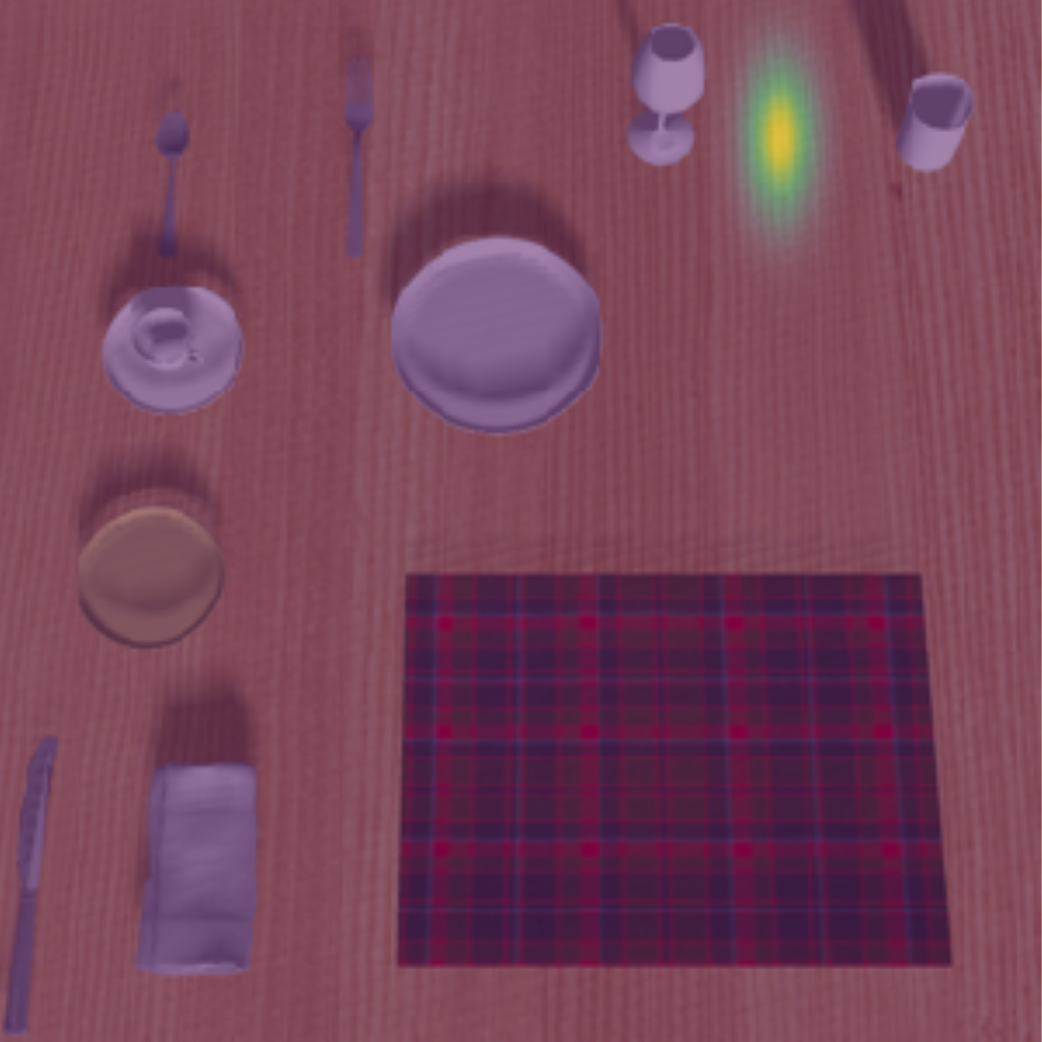} \\\midrule
Expert Demonstration & \includegraphics[width=0.3\textwidth]{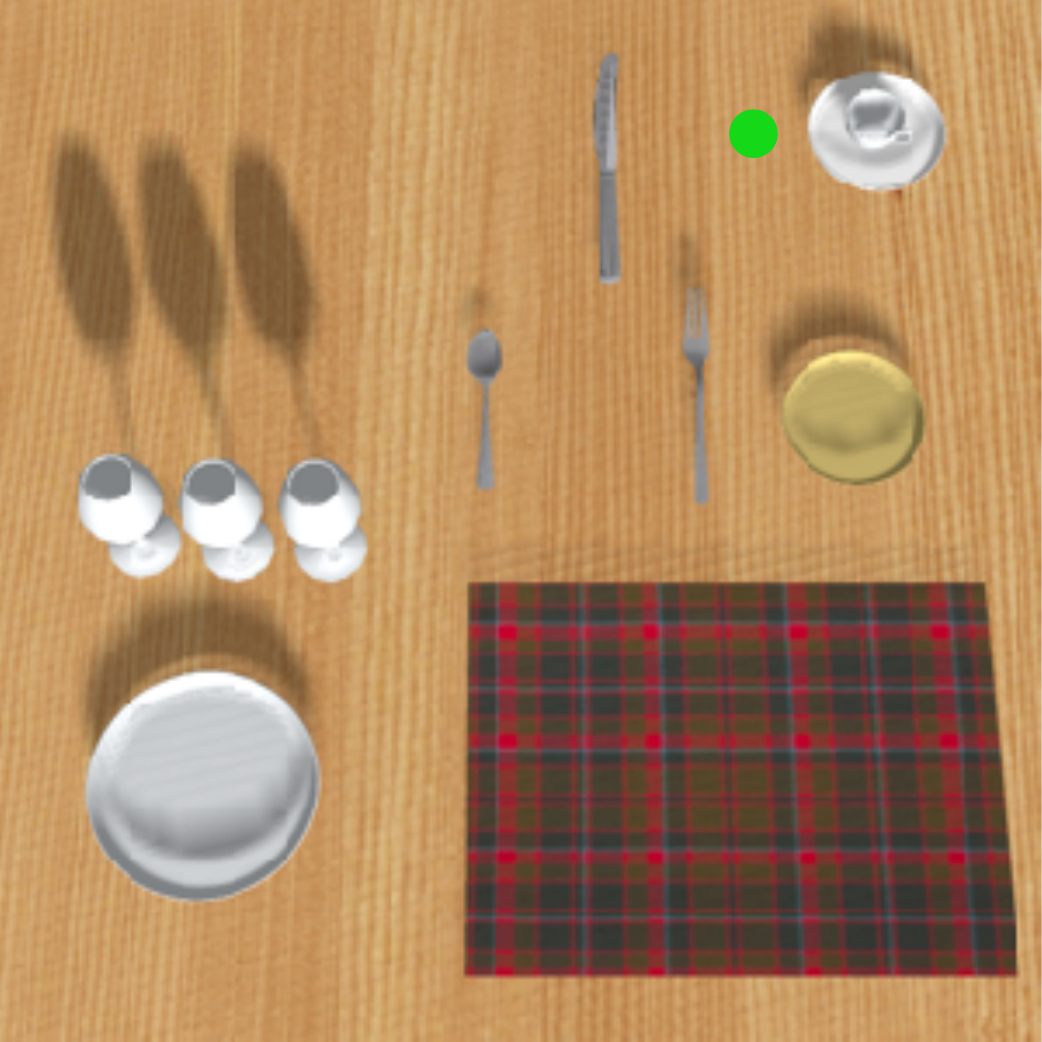} & \includegraphics[width=0.3\textwidth]{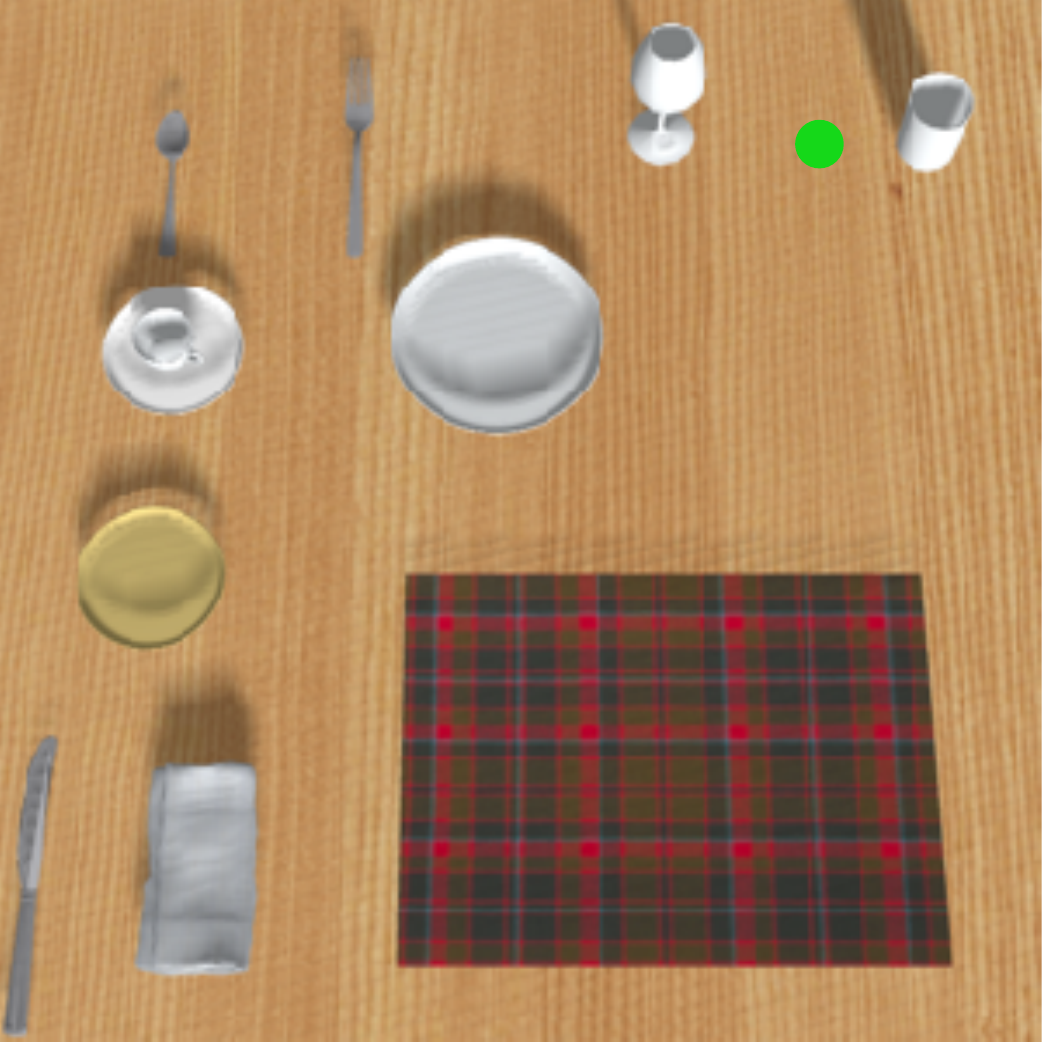} \\ \bottomrule
\end{tabular}
\caption{The examples of tasks in Tabletop Dataset.}
\label{app:tab_eg}
\end{table*}

\newpage
\section{Implementation and Training Details}
\label{app:implementation}

In this section, we introduce the implementation details of P\&G.

\subsection{Soft Parsing}

The architecture of soft parsing module is shown in Figure \ref{app:fig_soft_par_archi}. The pseudo-code of soft parsing is in Algorithm \ref{app:alg_soft_par}. 

\begin{figure*}[]
    \centering
    \includegraphics[width=0.8\textwidth]{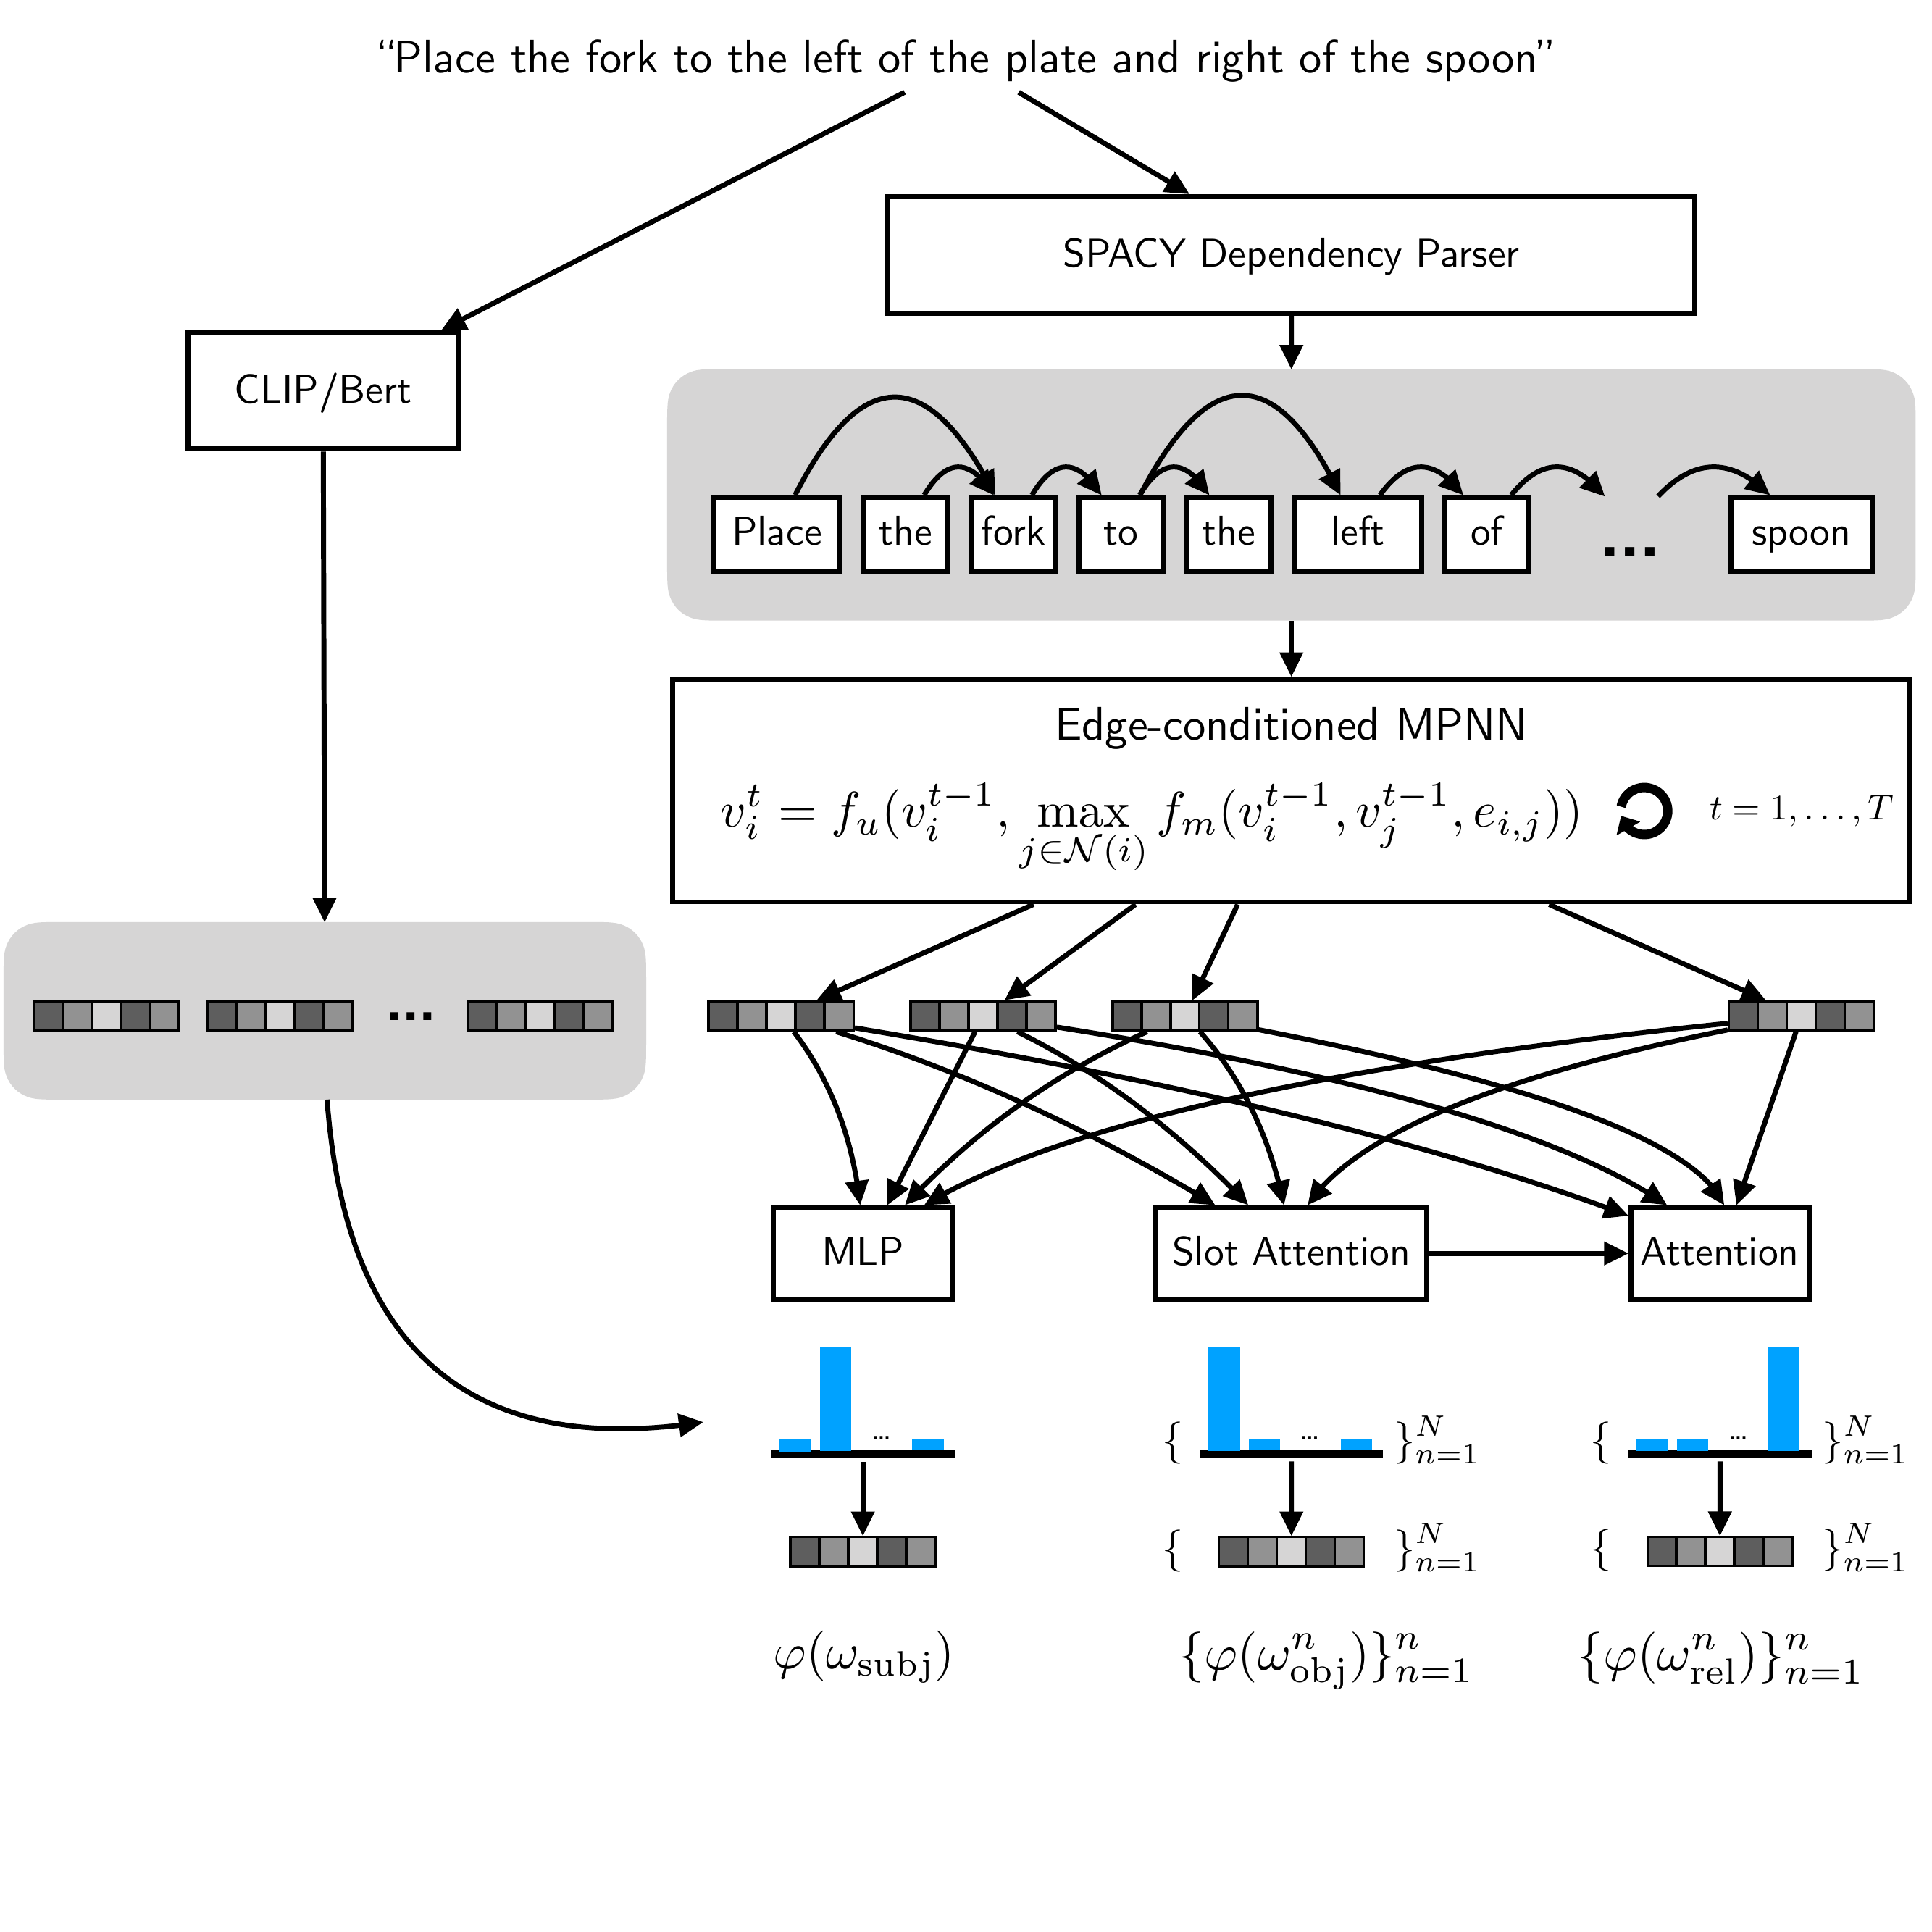}
    \caption{Soft Parsing implementation.}
    \label{app:fig_soft_par_archi}
\end{figure*}

\begin{algorithm}
\caption{Soft Parsing}
  \begin{algorithmic}[1]
    \INPUT Language instruction $\ell=\{\omega_l\}_{l=1}^L$, Language encoder $\phi(\cdot):\omega \rightarrow \mathbb{R}^{D_\text{word}}$, $K$
    \OUTPUT $\{(\varphi_\text{subj}, \varphi_\text{obj}^{(n)}, \varphi_\text{rel}^{(n)})\}_{n=1}^N$, $\tilde{\ell}$ 
    \STATE $\tau_\ell\leftarrow\mathrm{DepParser}(\ell)$
    \STATE $\{\varrho_l\}_{l=1}^L\leftarrow\mathrm{MPNN}(\tau_\ell) + \mathrm{CosinePositionEncoding}$
    \STATE $p(\omega_\text{subj})\leftarrow\mathrm{SoftMax}(\mathrm{MLP}(\{\varrho_l\}_{l=1}^L))$
    \STATE $\{p^{(n)}_\text{obj}(\omega_\text{obj})\}_{n=1}^N\leftarrow \mathrm{SlotAttention}(\{\varrho_l\}_{l=1}^L)$
    \STATE $\hat{\varrho}^{(n)}_\text{obj}\leftarrow\mathbb{E}_{p^{(n)}_\text{obj}}(\{\varrho_l\}_{l=1}^L)$
    \STATE $p^{(n)}_\text{rel}(\omega_\text{rel})\leftarrow\mathrm{MHAttn}(\{\hat{\varrho}^{(n)}_\text{obj}\}_{n=1}^N, \{\varrho_l\}_{l=1}^L, \{\varrho_l\}_{l=1}^L)$
    \STATE $\varphi_\text{subj}\leftarrow\mathbb{E}_{p_\text{subj}}(\{\phi_l\}_{l=1}^L)$, $\varphi^{(n)}_\text{obj}\leftarrow\mathbb{E}_{p^{(n)}_\text{obj}}(\{\phi_l\}_{l=1}^L)$, $\varphi^{(n)}_\text{rel}\leftarrow\mathbb{E}_{p^{(n)}_\text{rel}}(\{\phi_l\}_{l=1}^L)$
    \STATE $\forall\omega_l\in\ell, \tilde{\varphi}_l=\sum_{n=1}^N p^{(n)}_\mathrm{rel}(\omega_l)\cdot\varphi^{(n)}_\mathrm{rel}+
    \sum_{n=1}^N p^{(n)}_\mathrm{obj}(\omega_l)\cdot\varphi^{(n)}_\mathrm{obj}+
    p_\mathrm{subj}(\omega_l)\cdot\varphi_\mathrm{subj}$
    \STATE $\tilde{\ell}=\mathrm{LSTM}(\{\tilde{\varphi}_l\}_{l=1}^L)$
  \end{algorithmic}
 \label{app:alg_soft_par}
\end{algorithm}

\textbf{Structural Prior from Dependency Parsing.} We use SPACY dependency parser with transformer backend to get the dependency tree of a given sentence. We use embeddings $v\in\mathbb{R}^{D_\text{embed}}$ to represent the part-of-speech (POS) tag and dependency (DEP) tag in the dependency tree. The message passing neural network uses MLP as the functions $f_m: \mathbb{R}^{D_\text{embed}}\times\mathbb{R}^{D_\text{embed}}\times\mathbb{R}^{D_\text{embed}}\rightarrow\mathbb{R}^{D_\text{embed}}$ and $f_u: \mathbb{R}^{D_\text{embed}}\times\mathbb{R}^{D_\text{embed}}\rightarrow\mathbb{R}^{D_\text{embed}}$. The POS tags are used as the initial node features and the DEP tags are the edge attributes. During the message passing, the node features and/or edge attributes are concatenated as the input of $f_m$ and $f_u$. Thus, the structural prior from dependency tree are encoded in the output structural features of the message passing neural network. In addition, the structure lacks the order of position of the tokens in the sentence. We use cosine positional encoding added in the output structural embeddings to encode the position of tokens in the sentence. 

\textbf{Relation Extraction.} The output structural features $\varrho_l$ from the message passing neural network are used for relation extraction. We use attention to evaluate the normalized score of each token in the sentence from message passing for its contribution to the components in relational triplets. We use a single-layer MLP with softmax to compute the normalized score of each token contributing to the subject phrase. To discover potential object phrases, we use slot attention~\cite{locatello2020object} from visual object discovery for unsupervised object phrase discovery. The slot attention algorithm is illustrated in Algorithm \ref{app:alg_slot_attn}. After the object phrases are discovered, we use a two-layer multi-head attention module to evaluate the relational phrases conditioned on the corresponding object phrases. The object structure embeddings from slot attention are used as the query, and the structural features from message passing as the key and value. After we compute the weights of each token in the sentence for the subject phrase, object phrase, and relational phrase, we use the expected embedding to represent the word embeddings for the phrases in triplets. We use CLIP as the encoder to compute the word embeddings of tokens in the sentence.     

\begin{algorithm}
\caption{Slot Attention}
  \begin{algorithmic}[1]
    \INPUT $\mathrm{inputs}\in\mathbb{R}^{N\times D_\text{inputs}}, \mathrm{slots}\sim\mathcal{N}(\mu, \mathrm{diag}(\sigma))\in\mathbb{R}^{K\times D_\text{slots}}$
    \PARAM $k, q, v:$ linear projections for attention; $\mathrm{GRU}$; $\mathrm{MLP}$; $\mathrm{LayerNorm}(\times 3)$
    \STATE $\mathrm{inputs}\leftarrow\mathrm{LayerNorm}(\mathrm{inputs})$
    \FOR{$t=0, \ldots, T$}
        \STATE $\mathrm{slots\_prev} \leftarrow \mathrm{slots}$
        \STATE $\mathrm{slots} \leftarrow \mathrm{LayerNorm} (\mathrm{slots})$
        \STATE $\mathrm{attn}\leftarrow\mathrm{SoftMax}(\frac{1}{\sqrt{D}}k(\mathrm{inputs}) q(\mathrm{slots})^\top, \mathrm{axis}=\mathrm{slots})$
        \STATE $\mathrm{Updates}\leftarrow \mathrm{WeightedMean}(\mathrm{weights}=\mathrm{attn} + \epsilon, \mathrm{values}=v(\mathrm{inputs}))$
        \STATE $\mathrm{slots}\leftarrow \mathrm{GRU} (\mathrm{state}=\mathrm{slots\_prev}, \mathrm{inputs}=\mathrm{updates})$
        \STATE $\mathrm{slots} \leftarrow \mathrm{slots} +  \mathrm{MLP} (\mathrm{LayerNorm} (\mathrm{slots}))$ 
    \ENDFOR
    \OUTPUT $\mathrm{slots}$
  \end{algorithmic}
 \label{app:alg_slot_attn}
\end{algorithm}

\textbf{Hyper-parameters. }The dimension of embedding is $D_\text{embed}=64$, and the layer number of message passing neural network is 4. We use 3 iteration for slot attention, with slot number $N_\text{slot}=4$, hidden dimension $D_\text{slots}=128$ and $\epsilon=1\times10^{-8}$. As for the multi-head attention module for relational phrase discovery, the number of heads is 8 and embedding dimension is 64. Language encoder $\phi(\cdot)$ is pretrained CLIP (ViT-32/B), in which the word embedding dimension is $D_\text{word}=512$. 

\subsection{Particle Mean-field GNN}

The pseudo-code of particle mean-field GNN is illustrated in Algorithm \ref{app:alg_par_gnn}. 

\textbf{Functions in Particle Mean-field GNN.} For the observation, we use masks of bounding boxes to represent the object positions and shapes in the observed image. We use a simple CNN model $f_\Phi:\mathbb{R}^{W_\text{pos}\times H_\text{pos}} \rightarrow \mathbb{R}^{D_\text{pmpnn}}$ to encode the positional feature of the bounding boxes detected in the scene. The particle proposal network $f_\Psi:\mathbb{R}^{D_\text{pmpnn}}\times \mathbb{R}^{D_\text{pmpnn}} \rightarrow \mathbb{R}^{D_\text{pmpnn}}$ and aggregation network $f_u:\mathbb{R}^{D_\text{pmpnn}} \rightarrow \mathbb{R}^{D_\text{pmpnn}}$ are all single-layer MLP. We implement message perturbation by reparameterization trick. We model the Gaussian random variable by a learned mean and variance matrix: 
\begin{align}
    &\mathbf{h}_\mathrm{out} = W_\mu\mathbf{h}_\mathrm{in} + \mathbf{b}_\mu + \boldsymbol{\xi}\\
    & \boldsymbol{\xi} \sim \mathcal{N}(0, \boldsymbol{\Sigma})\\
    & \boldsymbol{\Sigma} = W_\Sigma\mathbf{h}_\mathrm{in} + \mathbf{b}_\Sigma
\end{align}

\textbf{Hyper-parameters. }The layer number of particle-based mean-field GNN is $T=8$. In message passing, we use embeddings with dimension $D_\text{pmpnn}=128$. In soft resampling, we use $\alpha = 0.5$. For visual grounding, the the visual encoder is pretrained CLIP (ViT-32/B).

\begin{algorithm}[]
\caption{Mean-field GNN}
  \begin{algorithmic}[1]
    \INPUT Number of layer $T$, detected object bounding boxes $\mathbf{B}=\{(\obs_m, \bfx_m)\}_{m=1}^M$, embeddings of relational triplets $\varphi(\Omega)=\{\langle\varphi_\text{subj}, \varphi_\text{rel}^{(n)}, \varphi_\text{obj}^{(n)}\rangle\}$
    \STATE $\mathbf{h}_{i}^{(0)}\leftarrow\mathbf{0},~t\leftarrow 0$\hfill\COMMENT{Initialization}
    \STATE $\forall i, {\mathbf{h}}_{\bfy, i, m}\leftarrow f_\Phi(\bfx_m)$
    \STATE ${w}_{\bfy, i, m}\leftarrow g_\Phi(\obs_m, \varphi(\omega_i)),~\omega_i\in\{\omega_\text{subj}, \omega^{(n)}_\text{obj}\}$
    \FOR{$t<T$}
        \STATE $\mathbf{h}_{\bfy, i} \leftarrow \sigma(\sum_m w_{\bfy,i,m}\mathbf{h}_{\bfy, i, m})$
        \FOR{$(i,j)\in\mathcal{E}$}\hfill\COMMENT{Message Computing}
            \STATE $\mathbf{m}_{j\to i}^{(t)} \leftarrow f_\Psi(\mathbf{h}_{j}^{(t-1)} + \mathbf{h}_{\bfy, j}, r_{i,j}), r_{i,j}\in\{\varphi^{(n)}_\text{rel}\}_{n=1}^N$
            \STATE $\mathbf{m}_{j\to i}^{(t)} \leftarrow\mathrm{LeakyReLU}(\mathbf{m}_{j\to i}^{(t)})$
        \ENDFOR
        \FOR{$i\in\mathcal{V}$}\hfill\COMMENT{Message Aggregation}
            \STATE $\tilde{\mathbf{h}}_{i}^{(t)}\leftarrow f_u(\mathbf{h}_{\bfy, i} + \sum_{j\in\mathcal{N}(i)}\mathbf{m}_{j\to i}^{(t)})$
            \STATE $\mathbf{h}_{i}^{(t)}\leftarrow\mathrm{LeakyReLU}(\tilde{\mathbf{h}}_{i}^{(t)})$
        \ENDFOR
        \STATE $t \leftarrow t + 1$
    \ENDFOR
    \OUTPUT $\{\mathbf{h}_{i}^{(T)}\}_i$ 
  \end{algorithmic}
  \label{app:alg_par_gnn}
\end{algorithm}

\begin{algorithm}[]
\caption{Particle Mean-field GNN}
  \begin{algorithmic}[1]
    \INPUT Number of layer $T$, number of particles $K$, detected object bounding boxes $\mathbf{B}=\{(\obs_m, \bfx_m)\}_{m=1}^M$, embeddings of relational triplets $\varphi(\Omega)=\{\langle\varphi_\text{subj}(\omega), \varphi(\omega_\text{rel}^{(n)}), \varphi(\omega_\text{obj}^{(n)})\rangle\}$
    \STATE $\mathbf{h}_{i,k}^{(0)}\sim\mathcal{N}(0, 1),~w_{i,k}^{(0)}\leftarrow 1/K,~t\leftarrow 0$\hfill\COMMENT{Initialization}
    \STATE $\forall i, \tilde{\mathbf{h}}_{\bfy, i, m}\leftarrow f_\Phi(\bfx_m)$
    \STATE $\tilde{w}_{\bfy, i, m}\leftarrow g_\Phi(\obs_m, \varphi(\omega_i)),~\omega_i\in\{\omega_\text{subj}, \omega^{(n)}_\text{obj}\}$
    \FOR{$t<T$}
        \STATE $\{(\mathbf{h}_{\bfy, i, k}, w_{\bfy, i, k})\}_{k=1}^K\leftarrow\mathrm{SoftResamp}(\{(\tilde{\mathbf{h}}_{\bfy, i, m}, \tilde{w}_{\bfy, i, m})\}_{m=1}^M)$
        \STATE $ \boldsymbol{\xi}^t_{\bfx, i, k}\sim\mathcal{N}\left[0, \boldsymbol{\Sigma}^t_{\bfx, i, k}(\mathbf{h}_{\bfy, i, k})\right]$
        \STATE $\mathbf{h}_{\bfy, i, k} \leftarrow \mathbf{h}_{\bfy, i, k} + \boldsymbol{\xi}^t_{\bfx, i, k}$
        \FOR{$(i,j)\in\mathcal{E}$}\hfill\COMMENT{Message Computing}
            \STATE $\boldsymbol{\xi}_{j}^t\sim\mathcal{N}[0, \boldsymbol{\Sigma}_j^t(\mathbf{h}_{j,k}^{(t-1)} + \mathbf{h}_{\bfy, j, k}, r_{i,j})]$
            \STATE $\mathbf{m}_{j\to i,k}^{(t)} \leftarrow f_\Psi(\mathbf{h}_{j,k}^{(t-1)} + \mathbf{h}_{\bfy, j, k}, r_{i,j}) + \boldsymbol{\xi}_{j}^t, r_{i,j}\in\{\varphi^{(n)}_\text{rel}(\omega)\}_{n=1}^N$
            \STATE $\mathbf{m}_{j\to i,k}^{(t)} \leftarrow\mathrm{LeakyReLU}(\mathbf{m}_{j\to i,k}^{(t)})$
            \STATE $w_{j\to i, k}^{(t)}\leftarrow w_{j,k}^{(t-1)}\log w_{\bfy, j, k}$
        \ENDFOR
        \FOR{$i\in\mathcal{V}$}\hfill\COMMENT{Message Aggregation}
            \STATE $\tilde{\mathbf{h}}_{i,k}^{(t)}\leftarrow f_u(\mathbf{h}_{\bfy, i, k} + \sum_{j\in\mathcal{N}(i)}\mathbf{m}_{j\to i, k}^{(t)})$
            \STATE $\tilde{\mathbf{h}}_{i,k}^{(t)}\leftarrow\mathrm{LeakyReLU}(\tilde{\mathbf{h}}_{i,k}^{(t)})$
            \STATE $\tilde{w}_{i,k}^{(t)}\leftarrow\eta w_{\bfy, i, k}\prod_{j\in\mathcal{N}(i)}w_{j\to i, k}^{(t)}$
            \STATE $\{(\mathbf{h}_{i,k}^{(t)}, w_{i,k}^{(t)})\}_{k=1}^K\leftarrow\mathrm{SoftResamp}(\{(\tilde{\mathbf{h}}_{i,k}^{(t)}, \tilde{w}_{i,k}^{(t)})\})$ 
        \ENDFOR
        \STATE $t \leftarrow t + 1$
    \ENDFOR
    \OUTPUT $\{(\mathbf{h}_{i,k}^{(T)}, w_{i,k}^{(T)})\}_k$ 
  \end{algorithmic}
  \label{app:alg_par_gnn}
\end{algorithm}

\subsection{Training}

We conduct supervised learning to train the model end-to-end. There are two components in the training objective. We first minimize the $L_2$ and $L_1$ loss between the prediction and groundtruth: $ \mathbb{E}(\mathcal{J}_{L_2})=\sum_kw_{i,k}^* (\bfy_{i,k}^*-\bfy_\text{gt})^2,~\mathbb{E}(\mathcal{J}_{L_1})=\sum_kw_{i,k}^* \|\bfy_{i,k}^*-\bfy_\text{gt}\|_1$. In order to implicitly learn the object grounding, we also use contrastive loss to increase the weight of particles nearest to the groundtruth while decreasing the weight of particles further away: $\mathcal{J}_\text{cont}=\log w_{i,k}^{*\min}-\log\sum_kw_{i,k}^*$. Thus, the learning objective is: $\mathcal{J}=\mathcal{J}_\text{cont} + \lambda_1 \mathbb{E}(\mathcal{J}_{L_2}) + \lambda_2\mathbb{E}(\mathcal{J}_{L_1})$. The hyper-parameter $\lambda_1=50.0$ and $\lambda_2=1.0$. For target object grounding, we use cross entropy loss, where the labels for the loss function is the closest bounding box to the ground truth object position. 

For training, we use Adam optimizer, and the learning rate is $1\times 10^{-4}$. We train the model for 200K steps when the data is larger than 1000, and 50K when trained by 300 data. 

\subsection{Baseline Implementation}

\subsubsection{Baseline P\&G}

The baseline P\&G implement soft parsing and particle-based mean-field GNN without soft resampling and message perturbation. Thus, it does not conduct step 5 and step 16 of Algorithm \ref{app:alg_par_gnn}. It also use message without message perturbation in step 6, 7 and step 9. Thus, it iteratively uses the message from neighboring nodes and observed nodes directly in step 2, 3, and 10.

\subsubsection{Baseline P\&G + Message Perturbation}

The second baseline is built upon the first baseline with message perturbation in step 6, 7 and step 9 of Algorithm \ref{app:alg_par_gnn}.

\subsubsection{Baseline P\&G + Soft Resampling}

The third baseline is built upon the first baseline with soft resampling in step 5 and step 16 of Algorithm \ref{app:alg_par_gnn}.

\subsubsection{P\&G without Soft Parsing}

This baseline model directly uses the embedding of the entire instruction sentence instead of the embeddings from triplets for grounding in step 3 and message passing in step 10 of Algorithm \ref{app:alg_par_gnn}.

\subsubsection{P\&G + ViT + Bert}

This baseline model uses ImageNet-pretrained ViT 32/B model for visual encoding, and pretrained Bert model for text encoding for visual grounding in step 3 of Algorithm \ref{app:alg_par_gnn}.

\subsection{Detailed Experimental Results}

We present the detailed experimental results without noise in observation in Appendix Table \ref{app:table_res1}. The details of experimental results with noisy observation are presented in Appendix Table \ref{app:table_res2}. During the discussion session, we will revise the experimental results of Table 2 in the paper.

\begin{table*}[h]
\footnotesize
\centering
\makebox[\textwidth][c]{
\begin{tabular}{{P{38mm}}*{6}{P{11mm}}*{3}{P{10mm}}}
    \toprule
    {\footnotesize \begin{tabular}[c]{@{}c@{}}Num of objects in scene\\\midrule Spatial Relation Type \end{tabular} } & 
    \multicolumn{3}{c}{\footnotesize \begin{tabular}[c]{@{}c@{}}4 Objects\\\midrule Single \end{tabular}} & 
    \multicolumn{3}{c}{\footnotesize \begin{tabular}[c]{@{}c@{}}10 Objects\\\midrule Single \end{tabular}} & 
    \multicolumn{3}{c}{\footnotesize \begin{tabular}[c]{@{}c@{}}10 Objects with Ambiguity\\\midrule Single \end{tabular}} \\ \cmidrule(lr){1-1}\cmidrule(lr){2-4}\cmidrule(lr){5-7}\cmidrule(lr){8-10}
    {Training Data Num}&{\footnotesize 300} &{\footnotesize 3k} &{\footnotesize 20k} &{\footnotesize 300} &{\footnotesize 3k} &{\footnotesize 20k}&{\footnotesize 300} &{\footnotesize 3k} &{\footnotesize 20k} \\ \cmidrule(lr){1-10} 
    %------
    
    CLIPort~\cite{shridhar2021cliport} & 41.1  & 84.8  & 92.3  & 39.1  & 78.0  & 84.1  & 37.7  & 76.4   & 82.0 \\
    P\&G & \textbf{79.2}  & 93.1  & 97.8  & \textbf{74.6}  & 85.2  & \textbf{95.1}  & \textbf{69.7}  & 86.5   & \textbf{88.9}  \\\cmidrule(lr){1-10} 
    P\&G (ViT+Bert) & 72.6  & \textbf{95.8}  & \textbf{97.9}  & 60.8  & \textbf{91.1}  & 95.0  & 60.5  & 85.7   & 87.9  \\
    P\&G (CLIP, w/o SP) & 59.3  & 87.4  & 89.5  & 56.2  & 77.2  & 83.3  & 51.1  & 78.1   & 80.3  \\\cmidrule(lr){1-10} 
    Baseline P\&G (w/o RS, RP) & 75.9  & 89.6  & 93.5  & 64.3  & 84.2  & 90.4  & 66.1  & 82.3   & 85.6  \\
    Baseline P\&G + RS & 78.0  & 92.9  & 97.2  & 69.9  & 90.9  & 94.2  & 67.0  & \textbf{86.7}   & 88.7  \\
    Baseline P\&G + RP & 51.1  & 78.0  & 83.3  & 42.0  & 68.8  & 75.1  & 49.3  & 61.8   & 72.3  \\

    \bottomrule
    \toprule
    {\footnotesize \begin{tabular}[c]{@{}c@{}}Num of objects in scene\\\midrule Spatial Relation Type \end{tabular} } & 
    \multicolumn{3}{c}{\footnotesize \begin{tabular}[c]{@{}c@{}}4 Objects\\\midrule Compositional \end{tabular}} & 
    \multicolumn{3}{c}{\footnotesize \begin{tabular}[c]{@{}c@{}}10 Objects\\\midrule Compositional \end{tabular}} & 
    \multicolumn{3}{c}{\footnotesize \begin{tabular}[c]{@{}c@{}}10 Objects with Ambiguity\\\midrule Compositional \end{tabular}} \\ \cmidrule(lr){1-1}\cmidrule(lr){2-4}\cmidrule(lr){5-7}\cmidrule(lr){8-10}
    {Training Data Num}&{\footnotesize 300} &{\footnotesize 3k} &{\footnotesize 20k} &{\footnotesize 300} &{\footnotesize 3k} &{\footnotesize 20k}&{\footnotesize 300} &{\footnotesize 3k} &{\footnotesize 20k} \\ \cmidrule(lr){1-10} 
    %------
    
    CLIPort~\cite{shridhar2021cliport} & 40.7  & 77.8  & 83.1 & 39.2  & 71.9  & 77.5  & 30.8  &  69.9  & 78.1 \\
    P\&G & \textbf{77.7}  & 90.7  & \textbf{94.3}  & \textbf{60.2}  & \textbf{82.3}  & \textbf{89.2}  & \textbf{56.8}  & \textbf{83.2}   & \textbf{89.3}  \\\cmidrule(lr){1-10} 
    P\&G (ViT+Bert) & 62.7  & \textbf{91.2}  & 93.0  & 57.3  & 82.1  & 86.3  & 56.5  & 78.2   & 81.8  \\
    P\&G (w/o SP) & 43.1  & 87.1  & 88.3  & 41.3  & 67.2  & 69.4  & 39.0  & 69.1   & 71.0  \\\cmidrule(lr){1-10} 
    Baseline P\&G (w/o RS, RP) & 67.2  & 86.0  & 91.7  & 51.2  & 76.3  & 83.4  & 40.2  & 78.9   & 83.8  \\
    Baseline P\&G + RS & 70.8  & 89.9  & 90.2  & 55.4  & \textbf{82.3}  & 85.9  & 51.1  & 78.5   & 81.3  \\
    Baseline P\&G + RP & 40.2  & 71.1  & 74.2  & 48.1  & 68.8  & 71.2  & 44.0  & 62.1   & 68.7  \\

    \bottomrule
\end{tabular}}
\caption{The detailed experimental results by clean observation for baselines and full design of P\&G, as well as CLIPort.}
\label{app:table_res1}
\end{table*}

The experimental results show that our approach is more sample-efficient and accurate than CLIPort for language-conditioned object placement when the language instructions are conditioned on compositional and ambiguous spatial relations. When trained by equal number of data, P\&G performs better than CLIPort in all tasks, especially when the model is trained by relatively small number of data, revealing the sample efficiency of P\&G. 

\begin{table*}[h]
\footnotesize
\centering
\makebox[\textwidth][c]{
\begin{tabular}{P{40mm}P{11mm}P{18mm}P{11mm}P{18mm}P{11mm}P{18mm}}

    \toprule
    {\footnotesize Num of objects in scene} & 
    \multicolumn{2}{c}{\footnotesize 4 Objects} & 
    \multicolumn{2}{c}{\footnotesize 10 Objects} & 
    \multicolumn{2}{c}{\footnotesize 10 Objects with Ambiguity} \\ \cmidrule(lr){1-1}\cmidrule(lr){2-3}\cmidrule(lr){4-5}\cmidrule(lr){6-7}
    {Spatial Relation Type}&{\footnotesize Single} &{\footnotesize Compositional} &{\footnotesize Single} &{\footnotesize Compositional} &{\footnotesize Single} &{\footnotesize Compositional} \\ \cmidrule(lr){1-7} 
    %------
    P\&G New & \textbf{93.2}  & \textbf{92.7}  & \textbf{96.2}  & \textbf{91.4}  & \textbf{89.6}  & \textbf{86.8} \\
    P\&G & 92.2  & {89.7}  & {90.8}  & {81.0}  & {86.8}  & {80.3}    \\\cmidrule(lr){1-7} 
    P\&G (ViT+Bert) & {94.3}  & 88.6  & 90.3  & 77.3  & 84.2  & 76.8   \\
    P\&G (w/o SP) & 61.2  & 47.4  & 57.5  & 36.2  & 57.2  & 33.3    \\
    P\&G (1K Data) & 79.2  & 73.7  & 74.4  & 69.0  & 71.2  & 65.3    \\\cmidrule(lr){1-7} 
    Baseline P\&G (w/o MP \& RS) & 86.7  & 89.5  & 83.6  & 77.1  & 81.9  & 78.7    \\
    Baseline P\&G + MP & 76.9  & 85.5  & 71.4  & 71.0  & 69.4  & 70.7    \\
    Baseline P\&G + RS & 91.8  & 89.6  & 88.6  & 75.6  & 84.2  & 76.6    \\
    \bottomrule
\end{tabular}}
\caption{Detailed experimental results with noisy observation.}
\label{app:table_res2}
\end{table*}

\section{Example Pictures}
\label{app:examples}

The examples are shown in Figure \ref{app:fig_pag}, Figure \ref{app:fig_pag_2}, and Figure \ref{app:fig_cliport}, including example placements by CLIPort.

\begin{figure*}[h]
    \centering
    \makebox[\textwidth][c]{
    \includegraphics[width=1.0\textwidth]{figs/example_pag_simple.pdf}}
    \caption{Example placements by P\&G}
    \label{app:fig_pag}
\end{figure*}

\begin{figure*}[h]
    \centering
    \makebox[\textwidth][c]{
    \includegraphics[width=1.0\textwidth]{figs/example_p&g.pdf}}
    \caption{Example placements by P\&G}
    \label{app:fig_pag_2}
\end{figure*}

\begin{figure*}[h]
\makebox[\textwidth][c]{
    \centering
    \includegraphics[width=1.0\textwidth]{figs/cliport_demo.pdf}}
    \caption{Example placements by CLIPort}
    \label{app:fig_cliport}
\end{figure*}
