# Supplementary material for: Differentiable Parsing and Visual Grounding of Natural Language Instructions for Object Placement
Source: arXiv:2210.00215 source file (2023-03-13)
Supplement: Supplementary file 4 [file appendix.pdf]

## APPENDIX I TABLETOP DATASET

We extend the dataset from [bit.ly/ParaGonProj](https://bit.ly/ParaGonProj) with randomly sampled objects and generate placement from several sampled spatial relations.

### A. Objects

We sample 50 dining objects with different classes, colors, and shapes, including forks, knives, spoons, plates, wine cups, water cups, and napkin cloths. The visualization of objects is in Fig. 5 (a).

### B. Language Expressions

Our dataset draws samples from commonly used spatial relations with various language expressions. The spatial relations includes left, right, front, behind, on top of, and their compositions. We also have ternary spatial relation “between”. The language expressions for each spatial relations are illustrated in Table V.

### C. Data Generation

1) *Instruction Generation*: We generate the instructions according to language templates. The template for tasks with single spatial relation is illustrated below:

[verb phrase] + [subject phrase] (1)

+ [spatial relation phrase] + [object phrase]. (2)

If the language instruction contains compositional spatial relations, the template is:

[verb phrase] + [subject phrase] (3)

+ [spatial relation phrase 1] + [object phrase 1] (4)

+ “and” + [spatial relation phrase 2] + [object phrase 2]. (5)

The spatial relations are sampled from Table V, and the subject phrases and object phrases are sampled according to the object class, object colors, and shapes, such as “yellow square plate”. We sample the verb phrases uniformly as random from “put”, “place”, and “move”.

#### 2) Image Generation:

- **Camera Setup.** We use four cameras to capture the visual observation. Similar to the Raven simulator, there are three RGB-D cameras with resolutions of  $640 \times 480$  that are placed on the rectangular table’s top, left, and right, pointing towards the center (see (a), (b), and (c) in Figure 9). We also have an RGB camera with a resolution of  $640 \times 640$  placed at the top of the table (see (d) in Figure 9 for the example picture).
- **Rendering.** We use NVISII as the rendering interface to get the photorealistic pictures of the visual scene. We randomly sample the position of the lights and their colors to add difficulties. In addition, due to the random lighting conditions, the visual scenes contain various light reflections, hampering the visual grounding of natural language.

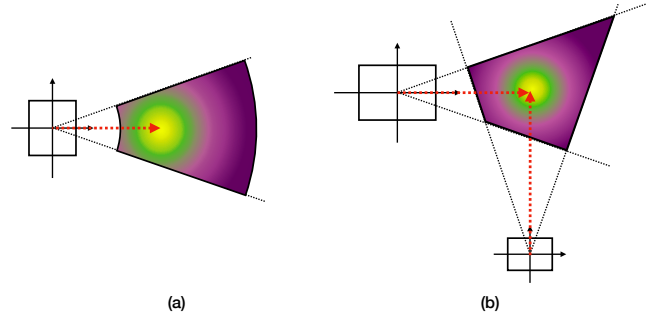

Fig. 8. Expert demonstration generation. The demonstration is sampled from a truncated Gaussian distribution. Case (a) illustrates a distribution of “left-hand side”, where the highlighted area indicates a high probability. We truncate areas that derive from the left side and are too close to the reference object. Case (b) illustrates the composition of spatial relations “left-hand side” and “upper side”, where the conjunction of both directions truncates the distribution.

3) *Expert Demonstration*.: We provide a handcrafted policy for expert demonstration in placement generation. According to the ground truth position of objects in the simulator, we sample from a handcrafted Gaussian distribution with a specific direction as the placement generation policy. Specifically, the demonstration is sampled from a truncated Gaussian distribution. There are two examples shown in Fig. 8. In this figure, case (a) illustrates a distribution of “left-hand side”, where the highlighted area indicates a high probability of placement. We truncate areas that derive from the left side and are too close to the reference object. Case (b) illustrates the composition of spatial relations “left-hand side” and “upper side”, where the conjunction of both directions truncates the distribution. The mean of the Gaussian distribution is located at the intersection of the central axes of the spatial relations. We also use axis-aligned bounding boxes (AABB) of the target object and context objects to detect intersections and avoid object collision after generating the placement.

### D. Evaluation Criteria

We evaluate the success rate of the object placing by examining whether the placement satisfies the spatial relational constraints in the natural language instructions. Specifically, we assess whether the generated particle is located at the truncated regions. For CLIPort, we take the argmax to get the generated placement. As ParaGon generates a set of particles as the samples of a placement distribution, we randomly sample from the particles ten times to evaluate the success rate.

## APPENDIX II IMPLEMENTATION AND TRAINING DETAILS

### A. Soft Parsing

We illustrate the implementation details of the soft parsing module. The algorithm is shown in Algorithm 3.

1) *Structural Prior from Dependency Parsing*: We use spaCy dependency parser with transformer backend to get the dependency tree of a given sentence. We use embeddings  $v \in \mathbb{R}^{D_{\text{embed}}}$  to represent the part-of-speech (POS) tag and dependency (DEP) tag in the dependency tree. The message passing neural network uses MLP as the functions  $f_m$  :

TABLE V  
SPATIAL RELATIONS AND THEIR LANGUAGE EXPRESSIONS IN TABLETOP DATASET.

| Spatial Relations | Language Expressions          | Spatial Relations | Language Expressions           |
|-------------------|-------------------------------|-------------------|--------------------------------|
| Left              | “to the left of”              | Front Right       | “to the lower right of”        |
|                   | “to the left side of”         |                   | “to the lower right side of”   |
|                   | “to the left hand side of”    |                   | “to the lower right corner of” |
| Right             | “to the right of”             | Behind Left       | “to the upper left of”         |
|                   | “to the right side of”        |                   | “to the upper left side of”    |
|                   | “to the right hand side of”   |                   | “to the upper left corner of”  |
| Front             | “in front of”                 | Behind Right      | “to the upper right of”        |
|                   | “to the lower side of”        |                   | “to the upper right side of”   |
| Behind            | “behind”                      | on top of         | “to the upper right corner of” |
|                   | “to the upper side of”        |                   | “on”                           |
| Front Left        | “to the lower left of”        |                   | “above”                        |
|                   | “to the lower left side of”   |                   | “on top of”                    |
|                   | “to the lower left corner of” |                   | “on the center of”             |
|                   | “to the front left of”        |                   |                                |

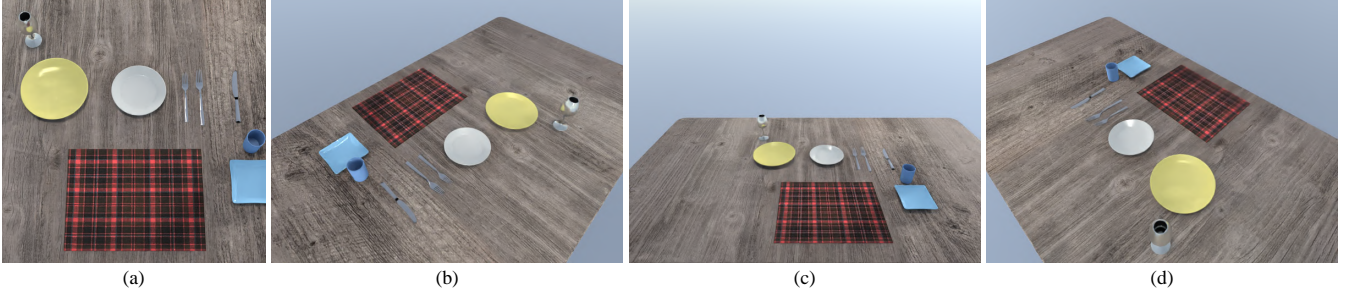

Fig. 9. Raw observations captured by cameras in Tabletop Dataset.

#### Algorithm 1 Soft Parsing

**Input:** Instruction  $\ell = \{\omega_l\}_{l=1}^L$ , Text encoder  $f_{\text{CLIP}}(\cdot) : \omega \rightarrow \mathbb{R}^{D_{\text{word}}}, K$

**Output:** Triplets:  $\{(\varphi_{\text{subj}}, \varphi_{\text{obj}}^{(n)}, \varphi_{\text{rel}}^{(n)})\}_{n=1}^N$ , Recovered instruction:  $\tilde{\ell}$

- 1:  $\tau \leftarrow \text{DepParser}(\ell)$
- 2:  $\{h_l\}_{l=1}^L \leftarrow \text{GNN}(\tau)$
- 3:  $\{a_{\text{subj}, l}\}_{l \leq L} \leftarrow \text{SoftMax}(\text{MLP}(\{h_l\}_{l=1}^L))$
- 4:  $\{a_{\text{obj}, l}^n\}_{n \leq N, l \leq L} \leftarrow \text{SlotAttn}(\{h_l\}_{l=1}^L)$
- 5:  $\tilde{h}_{\text{obj}}^n \leftarrow \sum_l a_{\text{obj}, l}^n h_l$
- 6:  $\{a_{\text{obj}, l}^n\}_{n \leq N, l \leq L} \leftarrow \text{MHAttn}(\{\tilde{h}_{\text{obj}}^n\}_{n=1}^N, \{h_l\}_{l=1}^L, \{h_l\}_{l=1}^L)$
- 7:  $\varphi_{\text{subj}} \leftarrow \sum_l a_{\text{subj}, l} f_{\text{CLIP}}(\omega_l)$
- 8:  $\varphi_{\gamma}^n \leftarrow \sum_l a_{\gamma, l}^n f_{\text{CLIP}}(\omega_l), \gamma \in \{\text{obj}, \text{rel}\}$
- 9:  $\tilde{\varphi}_l = \sum_{n=1}^N \sum_{i \in \{\text{rel}, \text{obj}\}} a_{i, l}^n \varphi_i^n + a_{\text{subj}, l} \varphi_{\text{subj}}$
- 10:  $\tilde{\ell} = \text{LSTM}(\{\tilde{\varphi}_l\}_{l=1}^L)$

$\mathbb{R}^{D_{\text{embed}}} \times \mathbb{R}^{D_{\text{embed}}} \times \mathbb{R}^{D_{\text{embed}}} \rightarrow \mathbb{R}^{D_{\text{embed}}}$  and  $f_u : \mathbb{R}^{D_{\text{embed}}} \times \mathbb{R}^{D_{\text{embed}}} \rightarrow \mathbb{R}^{D_{\text{embed}}}$ . The POS tags are used as the initial node features and the DEP tags are the edge attributes. During the message passing, the node features and edge attributes are concatenated as the input of  $f_m$  and  $f_u$ . Thus, the structural prior from the dependency tree is encoded in the output structural features of the message-passing neural network. In addition, the structure lacks the order of position of the

tokens in the sentence. We use cosine positional encoding added in the output structural embeddings to encode the position of tokens in the sentence.

2) *Relation Extraction:* The output structural features  $h_l$  from the message-passing neural network are used for relation extraction. We use attention to evaluate the normalized score of each token in the sentence from message passing for its contribution to the components in relational triplets. We use a single-layer MLP with softmax to compute the normalized score of each token contributing to the subject phrase. To discover potential object phrases, we use slot attention [35] from visual object discovery for unsupervised object phrase discovery. The slot attention algorithm is illustrated in Algorithm 2. After discovering the object phrases, we use a multi-head attention module to evaluate the relational phrases conditioned on the corresponding object phrases. The object structure embeddings from slot attention are used as the query, and the structural features from message passing as the key and value. After we compute the weights of each token in the sentence for the subject phrase, object phrase, and relational phrase, we use the expected embedding to represent the word embeddings for the phrases in triplets. We use CLIP as the encoder to compute the word embeddings of tokens in the sentence.

3) *Hyper-parameters*: The dimension of embedding is  $D_{\text{embed}} = 64$ , and the layer number of message passing neural network is 4. We use 3 iteration for slot attention, with slot number  $N_{\text{slot}} = 4$ , hidden dimension  $D_{\text{slots}} = 128$  and  $\epsilon = 1 \times 10^{-8}$ . As for the multi-head attention module for relational phrase discovery, the number of heads is eight, and the embedding dimension is 64. Language encoder  $\phi(\cdot)$  is trained CLIP (ViT-32/B), in which the word embedding dimension is  $D_{\text{word}} = 512$ .

---

#### Algorithm 2 Slot Attention

---

**Input:** inputs  $\in \mathbb{R}^{N \times D_{\text{inputs}}}$ , slots  $\sim \mathcal{N}(\mu, \text{diag}(\sigma)) \in \mathbb{R}^{K \times D_{\text{slots}}}$

**Layer params:**  $k, q, v$  : linear projections for attention; GRU; MLP; LayerNorm( $\times 3$ )

```

1: inputs  $\leftarrow$  LayerNorm(inputs)
2: for  $t = 0, \dots, T$  do
3:   slots_prev  $\leftarrow$  slots
4:   slots  $\leftarrow$  LayerNorm(slots)
5:   attn  $\leftarrow$  SoftMax( $\frac{1}{\sqrt{D}} k(\text{inputs}) q(\text{slots})^\top$ , axis = slots)
6:   Updates  $\leftarrow$  WeightedMean(weights = attn +  $\epsilon$ , values =  $v(\text{inputs})$ )
7:   slots  $\leftarrow$  GRU(state = slots_prev, inputs = updates)
8:   slots  $\leftarrow$  slots + MLP(LayerNorm(slots))
9: end for

```

**Output:** slots

---

### B. Particle Mean-field GNN

The pseudo-code of particle mean-field GNN is illustrated in Algorithm 3.

1) *Functions in Particle Mean-field GNN*: For the observation, we use masks of bounding boxes to represent the object positions and shapes in the observed image. We use a simple CNN model  $f_{\text{pos}} : \mathbb{R}^{W_{\text{pos}} \times H_{\text{pos}}} \rightarrow \mathbb{R}^{D_{\text{mpnn}}}$  to encode the positional feature of the bounding boxes detected in the scene. We then use an MLP to project the positional feature into embeddings. The particle proposal network  $f_\psi : \mathbb{R}^{D_{\text{mpnn}}} \times \mathbb{R}^{D_{\text{mpnn}}} \rightarrow \mathbb{R}^{D_{\text{mpnn}}}$  and aggregation network  $f_u : \mathbb{R}^{D_{\text{mpnn}}} \rightarrow \mathbb{R}^{D_{\text{mpnn}}}$  are all single-layer MLP. The reweighting function of observation model  $g_\phi : \mathbb{R}^{D_{\text{mpnn}}} \times \mathbb{R}^{D_{\text{mpnn}}} \rightarrow \mathbb{R}$  is also a MLP.

2) *Hyper-parameters*: The layer number of particle-based mean-field GNN is  $T = 8$ . In message passing, we use embeddings with dimension  $D_{\text{mpnn}} = 128$ . In soft resampling, we use  $\alpha = 0.5$  for training and  $\alpha = 1.0$  for inference. For visual grounding, the visual encoder is pre-trained CLIP (ViT-32/B).

### C. Training

We conduct supervised learning to train the model end-to-end. There are two components to the training objective. One is the negative log-likelihood of dataset  $\bar{\mathcal{X}}$ :  $\mathcal{J}_l = \sum_{\bar{\mathbf{x}} \in \bar{\mathcal{X}}} -\log \sum_k w_k^* \mathcal{N}(\bar{\mathbf{x}}; \mathbf{x}_k^*, \Sigma)$ , where  $\bar{\mathbf{x}} \in \bar{\mathcal{X}}$  is the labeled placement and the likelihood is a mixture of Gaussian represented by each output particle of target object

---

### Algorithm 3 Particle Mean-field GNN

---

**Input:** Number of layer  $T$ , number of particles  $K$ , detected object bounding boxes  $\mathbf{B} = \{(\mathbf{o}_m, \mathbf{x}_m)\}_{m=1}^M$ , relational graph  $\mathcal{G} = (\mathcal{V}, \mathcal{E})$ , edge attributes (spatial relation embeddings)  $r_{ij}$

```

1:  $h_{i,k}^{(0)} \sim \mathcal{N}(0, 1)$ ,  $w_{i,k}^{(0)} \leftarrow 1/K$ ,  $t \leftarrow 0$  {Initialization}
2: for  $t < T$  do
3:   for  $(i, j) \in \mathcal{E}$  do {Message Computing}
4:      $m_{ji,k}^t = f_\psi(h_{j,k}^{t-1}, r_{ij})$ 
5:      $m_{\text{obs},j}^t = f_\phi(\sum_{m=1}^M b_m^j f_{\text{pos}}(\mathbf{y}_m))$ 
6:      $w_{ji,k}^t = \eta w_{j,k}^{t-1} \log g_\phi(h_{j,k}^{t-1}, m_{\text{obs},j}^t)$ 
7:   end for
8:   for  $i \in \mathcal{V}$  do {Message Aggregation}
9:      $h_{i,k}^t = f_u(\sum_{j \in N(i)} m_{ji,k}^t + m_{\text{obs},i}^t)$ 
10:     $\log w_{i,k}^t = c + \log g_\phi(h_{i,k}^t, m_{\text{obs},i}^t) + \sum_{j \in N(i)} w_{ji,k}^t$ 
11:     $\{(h_{i,k}^t, w_{i,k}^t)\}_{k=1}^K \leftarrow \text{SoftResam}(\{(h_{i,k}^t, w_{i,k}^t)\}_{k=1}^K)$ 
12:  end for
13:   $t \leftarrow t + 1$ 
14: end for
15:  $x_{i,k}^* = \pi_{\text{dec}}(h_{i,k}^T), \forall k \leq K$  {Decode Placement}

```

**Output:**  $\{(x_{i,k}^*, w_{i,k}^T)\}_{k=1}^K$

---

$\{(\mathbf{x}_k^*, w_k^*)\}_{k=1}^K$ . We also minimize the auxiliary loss for improving soft parsing:  $\mathcal{J}_s = \sum_{\ell \in \bar{\mathcal{X}}} \|\ell - \tilde{\ell}\|^2 = \sum_{\ell \in \bar{\mathcal{X}}} \sum_l (\omega_l - \tilde{\omega}_l)^2$ . As such, the final objective is:  $\mathcal{J} = \mathcal{J}_l + \lambda \mathcal{J}_s$ , where  $\lambda$  is a hyper-parameter. The hyper-parameter  $\lambda = 10.0$ . For target object grounding, we use cross-entropy loss, where the labels for the loss function are the closest bounding box to the ground truth object position.

For training, we use Adam optimizer, and the learning rate is  $1 \times 10^{-4}$ . We train the model for 200K steps when the data is more significant than 1000 and 50K when trained by 300.

### D. Baseline Implementation

1) *No Soft Parsing*: This baseline model directly uses the embedding of the entire instruction sentence instead of the embeddings from triplets for object grounding and message passing in step 4 of Algorithm 3.

2) *No Particle*: This baseline model does not have particles in the message passing, and the initially hidden features in step 1 of Algorithm 3 are vectors with zero values. It also does not have step 11 for soft parsing.

3) *No Resampling*: The third baseline is built without soft resampling in step 11 of Algorithm 3.

4) *PARAGON(ViT + Bert)*: This baseline model uses the ImageNet-pretrained ViT 32/B model for visual encoding and the pretrained Bert model for text encoding in visual grounding, representing the edge attribute  $r_{ij}$ .
